# Supplementary material for: Choosing the correlation structure of mixed effect models for experiments with stimuli
Source: arXiv:1903.10766 ancillary file (2020-10-16)
Supplement: Supplementary file 1 [file matsup.pdf]

# Choosing the correlation structure of mixed effect models for experiments with stimuli: Supplementary material

Jaromil Frossard & Olivier Renaud

27-08-2020

# 1 Results of simulation: type I error rate

## 1.1 Design M1

Table S1: Type I error rate of the design M1 (see Table 2): The data are simulated using spherical random effects, 18 participants, and 18 stimuli. Represented are the models that include random effects associated to the interaction participants:stimuli.

| | | RI+ | RI-L+ | MAX+ | ZCP-sum+ | ZCP-poly+ | gANOVA+ | CS-PCA+ |
|---|---|---|---|---|---|---|---|---|
| Ap | no PT:SM | .082 | **.050** | **.050** | **.050** | **.050** | **.050** | **.050** |
| | | [.074;.091] | **[.043;.057]** | **[.043;.057]** | **[.043;.057]** | **[.043;.057]** | **[.043;.057]** | **[.043;.057]** |
| | PT:SM | .082 | **.050** | **.050** | **.050** | **.050** | **.050** | **.050** |
| | | [.074;.091] | **[.043;.057]** | **[.043;.057]** | **[.043;.057]** | **[.043;.057]** | **[.043;.057]** | **[.043;.057]** |
| As | no PT:SM | .086 | **.049** | **.049** | **.049** | **.049** | **.049** | **.049** |
| | | [.078;.095] | **[.043;.056]** | **[.043;.056]** | **[.043;.056]** | **[.043;.056]** | **[.043;.056]** | **[.043;.056]** |
| | PT:SM | .088 | **.049** | **.049** | **.049** | **.049** | **.049** | **.049** |
| | | [.080;.098] | **[.043;.056]** | **[.043;.057]** | **[.043;.056]** | **[.043;.056]** | **[.043;.056]** | **[.043;.056]** |
| Am | no PT:SM | .378 | **.050** | **.050** | **.050** | **.050** | **.050** | **.056** |
| | | [.363;.393] | **[.043;.057]** | **[.043;.057]** | **[.044;.058]** | **[.044;.058]** | **[.044;.058]** | **[.049;.064]** |
| | PT:SM | .387 | **.050** | **.050** | **.050** | **.050** | **.050** | **.053** |
| | | [.372;.403] | **[.043;.057]** | **[.043;.057]** | **[.043;.057]** | **[.043;.057]** | **[.043;.057]** | **[.046;.060]** |
| Ap:As | no PT:SM | .408 | **.049** | **.048** | **.048** | **.048** | **.048** | **.048** |
| | | [.393;.423] | **[.043;.056]** | **[.042;.055]** | **[.042;.055]** | **[.042;.055]** | **[.042;.055]** | **[.042;.055]** |
| | PT:SM | .461 | **.049** | **.048** | **.049** | **.048** | **.048** | **.049** |
| | | [.446;.476] | **[.043;.056]** | **[.042;.055]** | **[.042;.056]** | **[.042;.056]** | **[.042;.056]** | **[.043;.056]** |
| Ap:Am | no PT:SM | .308 | **.050** | **.048** | **.049** | **.049** | **.049** | .076 |
| | | [.294;.322] | **[.044;.058]** | **[.042;.055]** | **[.043;.056]** | **[.043;.056]** | **[.043;.056]** | [.069;.085] |
| | PT:SM | .319 | **.050** | **.048** | **.049** | **.049** | **.049** | .070 |
| | | [.305;.334] | **[.043;.057]** | **[.042;.055]** | **[.043;.056]** | **[.043;.056]** | **[.043;.056]** | [.062;.078] |
| As:Am | no PT:SM | .271 | **.048** | **.046** | **.047** | **.047** | **.047** | .070 |
| | | [.258;.285] | **[.042;.055]** | **[.040;.053]** | **[.041;.054]** | **[.041;.054]** | **[.041;.054]** | [.063;.079] |
| | PT:SM | .283 | **.047** | **.046** | **.046** | **.046** | **.046** | .067 |
| | | [.270;.298] | **[.041;.054]** | **[.040;.053]** | **[.040;.053]** | **[.040;.053]** | **[.040;.053]** | [.060;.075] |
| Ap:As:Am | no PT:SM | .162 | **.048** | **.044** | **.048** | **.048** | **.048** | .167 |
| | | [.151;.174] | **[.042;.055]** | **[.038;.051]** | **[.042;.055]** | **[.042;.055]** | **[.042;.055]** | [.156;.179] |
| | PT:SM | .171 | **.047** | **.045** | **.048** | **.048** | **.048** | .162 |
| | | [.159;.183] | **[.041;.054]** | **[.039;.052]** | **[.042;.055]** | **[.042;.055]** | **[.042;.055]** | [.151;.174] |

Table S2: Estimated type I error rate of the model M1 (see Table 2): The data are simulated using correlated random effects, 18 participants, and 18 stimuli. Represented are the models that do not include random effects associated to the interaction participants:stimuli.

| | | RI | RI-L | MAX | ZCP-sum | ZCP-poly | gANOVA | CS-PCA |
|---|---|---|---|---|---|---|---|---|
| Ap | no PT:SM | .076 | **.050** | **.049** | **.051** | **.050** | **.050** | **.051** |
| | | [.068;.084] | **[.043;.057]** | **[.043;.057]** | **[.044;.058]** | **[.044;.058]** | **[.044;.058]** | **[.045;.059]** |
| | PT:SM | .076 | **.047** | **.045** | **.047** | **.047** | **.047** | **.048** |
| | | [.068;.085] | **[.041;.054]** | **[.039;.053]** | **[.041;.054]** | **[.041;.054]** | **[.041;.054]** | **[.042;.055]** |
| As | no PT:SM | .087 | **.046** | **.044** | **.046** | **.046** | **.046** | **.047** |
| | | [.078;.096] | **[.040;.053]** | **[.038;.051]** | **[.040;.053]** | **[.040;.053]** | **[.040;.053]** | **[.041;.054]** |
| | PT:SM | .093 | **.049** | **.048** | **.050** | **.050** | **.050** | **.051** |
| | | [.084;.102] | **[.043;.056]** | **[.041;.055]** | **[.043;.057]** | **[.043;.057]** | **[.043;.057]** | **[.044;.058]** |
| Am | no PT:SM | .336 | **.053** | **.046** | **.053** | **.053** | **.053** | .281 |
| | | [.321;.350] | **[.047;.061]** | **[.040;.053]** | **[.047;.060]** | **[.046;.060]** | **[.046;.060]** | [.267;.295] |
| | PT:SM | .378 | **.050** | **.044** | **.050** | **.050** | **.050** | .212 |
| | | [.363;.393] | **[.044;.057]** | **[.038;.051]** | **[.043;.057]** | **[.043;.057]** | **[.043;.057]** | [.200;.226] |
| Ap:As | no PT:SM | .444 | **.050** | **.047** | **.049** | **.049** | **.049** | **.051** |
| | | [.429;.460] | **[.044;.058]** | **[.041;.054]** | **[.043;.056]** | **[.043;.056]** | **[.043;.056]** | **[.045;.058]** |
| | PT:SM | .494 | **.051** | **.048** | **.051** | **.050** | **.050** | **.052** |
| | | [.479;.510] | **[.045;.058]** | **[.042;.056]** | **[.044;.058]** | **[.044;.058]** | **[.044;.058]** | **[.046;.059]** |
| Ap:Am | no PT:SM | .250 | **.052** | *.040* | **.052** | **.052** | **.052** | .246 |
| | | [.237;.264] | **[.046;.060]** | *[.034;.047]* | **[.045;.059]** | **[.046;.060]** | **[.046;.060]** | [.233;.259] |
| | PT:SM | .286 | **.049** | *.041* | **.049** | **.049** | **.049** | .233 |
| | | [.273;.301] | **[.043;.056]** | *[.035;.048]* | **[.043;.056]** | **[.043;.056]** | **[.043;.056]** | [.220;.246] |
| As:Am | no PT:SM | .237 | **.052** | *.039* | **.052** | **.052** | **.052** | .237 |
| | | [.224;.250] | **[.046;.060]** | *[.033;.046]* | **[.046;.060]** | **[.046;.060]** | **[.046;.060]** | [.224;.250] |
| | PT:SM | .275 | **.053** | **.046** | **.053** | **.053** | **.053** | .222 |
| | | [.261;.289] | **[.047;.061]** | **[.039;.053]** | **[.047;.061]** | **[.047;.061]** | **[.047;.061]** | [.210;.236] |
| Ap:As:Am | no PT:SM | .121 | **.049** | *.027* | **.047** | **.047** | **.047** | .160 |
| | | [.111;.132] | **[.043;.056]** | *[.023;.033]* | **[.041;.054]** | **[.041;.054]** | **[.041;.054]** | [.149;.172] |
| | PT:SM | .148 | **.047** | *.036* | **.047** | **.046** | **.046** | .199 |
| | | [.138;.160] | **[.041;.054]** | *[.030;.042]* | **[.040;.054]** | **[.040;.054]** | **[.040;.054]** | [.187;.212] |

Table S3: Type I error rate of the model M1 (see Table 2): The data are simulated using correlated random effects, 18 participants, and 18 stimuli. Represented are the models that include random effects associated to the interaction participants:stimuli.

| | | RI+ | RI-L+ | MAX+ | ZCP-sum+ | ZCP-poly+ | gANOVA+ | CS-PCA+ |
|---|---|---|---|---|---|---|---|---|
| Ap | no PT:SM | .076 | **.051** | **.050** | **.052** | **.052** | **.052** | **.052** |
| | | [.068;.084] | **[.045;.058]** | **[.044;.058]** | **[.046;.060]** | **[.046;.060]** | **[.046;.060]** | **[.046;.060]** |
| | PT:SM | .076 | **.047** | **.047** | **.047** | **.047** | **.047** | **.048** |
| | | [.068;.085] | **[.041;.054]** | **[.041;.054]** | **[.041;.054]** | **[.041;.054]** | **[.041;.054]** | **[.042;.055]** |
| As | no PT:SM | .087 | **.047** | **.044** | **.047** | **.047** | **.047** | **.047** |
| | | [.078;.096] | **[.041;.054]** | **[.038;.051]** | **[.041;.054]** | **[.041;.054]** | **[.041;.054]** | **[.041;.054]** |
| | PT:SM | .093 | **.050** | **.048** | **.050** | **.050** | **.050** | **.050** |
| | | [.084;.102] | **[.043;.057]** | **[.042;.056]** | **[.044;.057]** | **[.044;.057]** | **[.044;.057]** | **[.044;.058]** |
| Am | no PT:SM | .376 | **.052** | **.048** | **.051** | **.051** | **.051** | .240 |
| | | [.361;.391] | **[.045;.059]** | **[.042;.055]** | **[.045;.059]** | **[.045;.059]** | **[.045;.059]** | [.228;.254] |
| | PT:SM | .394 | **.050** | **.044** | **.050** | **.050** | **.050** | .205 |
| | | [.380;.410] | **[.044;.057]** | **[.038;.051]** | **[.043;.057]** | **[.043;.057]** | **[.043;.057]** | [.193;.218] |
| Ap:As | no PT:SM | .402 | **.052** | **.047** | **.050** | **.050** | **.050** | **.052** |
| | | [.387;.417] | **[.045;.059]** | **[.041;.055]** | **[.044;.058]** | **[.044;.058]** | **[.044;.058]** | **[.046;.060]** |
| | PT:SM | .480 | **.051** | **.050** | **.051** | **.051** | **.051** | **.052** |
| | | [.464;.495] | **[.045;.059]** | **[.043;.058]** | **[.044;.058]** | **[.044;.058]** | **[.044;.058]** | **[.046;.059]** |
| Ap:Am | no PT:SM | .290 | **.048** | *.041* | **.048** | **.048** | **.048** | .231 |
| | | [.277;.305] | **[.042;.055]** | *[.035;.048]* | **[.042;.055]** | **[.042;.055]** | **[.042;.055]** | [.219;.245] |
| | PT:SM | .300 | **.049** | *.043* | **.048** | **.048** | **.048** | .229 |
| | | [.286;.315] | **[.043;.056]** | *[.037;.050]* | **[.042;.056]** | **[.042;.056]** | **[.042;.056]** | [.216;.242] |
| As:Am | no PT:SM | .283 | **.046** | *.038* | **.046** | **.046** | **.046** | .226 |
| | | [.269;.297] | **[.040;.054]** | *[.033;.045]* | **[.040;.054]** | **[.040;.054]** | **[.040;.054]** | [.213;.239] |
| | PT:SM | .289 | **.052** | **.048** | **.053** | **.053** | **.053** | .217 |
| | | [.275;.303] | **[.046;.060]** | **[.041;.055]** | **[.046;.060]** | **[.046;.060]** | **[.046;.060]** | [.205;.230] |
| Ap:As:Am | no PT:SM | .163 | **.044** | *.029* | *.043* | *.043* | *.043* | .180 |
| | | [.152;.175] | **[.039;.051]** | *[.024;.035]* | *[.037;.050]* | *[.037;.050]* | *[.037;.050]* | [.169;.193] |
| | PT:SM | .159 | **.046** | *.035* | **.046** | **.046** | **.046** | .200 |
| | | [.148;.171] | **[.040;.053]** | *[.030;.042]* | **[.040;.053]** | **[.040;.053]** | **[.040;.053]** | [.187;.212] |

Table S4: Type I error rate of the model M1 (see Table 2): The data are simulated using spherical random effects, 18 participants, and 36 stimuli. Represented are the models that include random effects associated to the interaction participants:stimuli.

| | | RI | RI-L | MAX | ZCP-sum | ZCP-poly | gANOVA | CS-PCA |
|---|---|---|---|---|---|---|---|---|
| Ap | no PT:SM | .068 | **.050** | **.051** | **.051** | **.051** | **.051** | **.051** |
| | | [.061;.077] | **[.043;.057]** | **[.045;.058]** | **[.045;.058]** | **[.045;.058]** | **[.045;.058]** | **[.045;.058]** |
| | PT:SM | .070 | **.051** | **.052** | **.052** | **.052** | **.052** | **.052** |
| | | [.062;.078] | **[.045;.059]** | **[.045;.059]** | **[.045;.059]** | **[.045;.059]** | **[.045;.059]** | **[.045;.059]** |
| As | no PT:SM | .144 | **.053** | **.053** | **.053** | **.053** | **.053** | **.053** |
| | | [.134;.156] | **[.046;.060]** | **[.046;.060]** | **[.046;.060]** | **[.046;.060]** | **[.046;.060]** | **[.046;.060]** |
| | PT:SM | .147 | **.054** | **.054** | **.054** | **.054** | **.054** | **.054** |
| | | [.137;.159] | **[.048;.062]** | **[.048;.062]** | **[.048;.062]** | **[.048;.062]** | **[.048;.062]** | **[.048;.062]** |
| Am | no PT:SM | .419 | **.051** | **.051** | **.050** | **.051** | **.050** | **.051** |
| | | [.404;.435] | **[.045;.058]** | **[.044;.058]** | **[.044;.058]** | **[.044;.058]** | **[.044;.058]** | **[.045;.058]** |
| | PT:SM | .462 | **.049** | **.049** | **.049** | **.049** | **.049** | **.049** |
| | | [.447;.478] | **[.043;.056]** | **[.043;.056]** | **[.043;.056]** | **[.043;.056]** | **[.043;.056]** | **[.043;.056]** |
| Ap:As | no PT:SM | .540 | **.051** | **.050** | **.050** | **.050** | **.050** | **.050** |
| | | [.525;.556] | **[.045;.058]** | **[.043;.057]** | **[.043;.057]** | **[.043;.057]** | **[.043;.057]** | **[.043;.057]** |
| | PT:SM | .571 | **.052** | **.051** | **.051** | **.051** | **.051** | **.052** |
| | | [.556;.587] | **[.046;.060]** | **[.045;.059]** | **[.045;.059]** | **[.045;.059]** | **[.045;.059]** | **[.045;.059]** |
| Ap:Am | no PT:SM | .380 | **.053** | **.052** | **.052** | **.052** | **.052** | .057 |
| | | [.365;.395] | **[.046;.060]** | **[.045;.059]** | **[.046;.059]** | **[.046;.059]** | **[.046;.059]** | [.050;.065] |
| | PT:SM | .424 | **.050** | **.050** | **.050** | **.050** | **.050** | **.052** |
| | | [.408;.439] | **[.044;.058]** | **[.043;.057]** | **[.043;.057]** | **[.043;.057]** | **[.043;.057]** | **[.045;.059]** |
| As:Am | no PT:SM | .278 | **.056** | **.055** | **.055** | **.055** | **.055** | .084 |
| | | [.264;.292] | **[.049;.063]** | **[.048;.062]** | **[.048;.063]** | **[.048;.063]** | **[.048;.063]** | [.076;.093] |
| | PT:SM | .323 | **.044** | **.044** | **.044** | **.044** | **.044** | .064 |
| | | [.309;.338] | **[.038;.051]** | **[.038;.051]** | **[.038;.051]** | **[.038;.051]** | **[.038;.051]** | [.057;.072] |
| Ap:As:Am | no PT:SM | .177 | .058 | **.056** | .057 | .057 | .057 | .148 |
| | | [.166;.189] | [.051;.065] | **[.049;.063]** | [.050;.065] | [.050;.065] | [.050;.065] | [.138;.160] |
| | PT:SM | .216 | **.052** | **.050** | **.051** | **.051** | **.051** | .109 |
| | | [.203;.229] | **[.045;.059]** | **[.044;.058]** | **[.045;.058]** | **[.045;.058]** | **[.045;.058]** | [.100;.119] |

Table S5: Type I error rate of the model M1 (see Table 2): The data are simulated using spherical random effects, 18 participants, and 36 stimuli. Represented are the models that include random effects associated to the interaction participants:stimuli.

| | | RI+ | RI-L+ | MAX+ | ZCP-sum+ | ZCP-poly+ | gANOVA+ | CS-PCA+ |
|---|---|---|---|---|---|---|---|---|
| Ap | no PT:SM | .068 | **.050** | **.051** | **.051** | **.051** | **.051** | **.051** |
| | | [.061;.077] | **[.044;.058]** | **[.045;.059]** | **[.045;.059]** | **[.045;.059]** | **[.045;.059]** | **[.045;.059]** |
| | PT:SM | .070 | **.051** | **.052** | **.052** | **.052** | **.052** | **.052** |
| | | [.062;.078] | **[.045;.059]** | **[.045;.059]** | **[.045;.059]** | **[.045;.059]** | **[.045;.059]** | **[.045;.059]** |
| As | no PT:SM | .144 | **.055** | **.055** | **.055** | **.055** | **.055** | **.055** |
| | | [.134;.156] | **[.048;.063]** | **[.048;.062]** | **[.048;.062]** | **[.048;.062]** | **[.048;.062]** | **[.048;.062]** |
| | PT:SM | .147 | **.054** | **.054** | **.054** | **.054** | **.054** | **.054** |
| | | [.137;.159] | **[.048;.062]** | **[.048;.062]** | **[.048;.062]** | **[.048;.062]** | **[.048;.062]** | **[.048;.062]** |
| Am | no PT:SM | .463 | **.049** | **.048** | **.048** | **.048** | **.048** | **.048** |
| | | [.448;.479] | **[.043;.056]** | **[.042;.055]** | **[.042;.055]** | **[.042;.055]** | **[.042;.055]** | **[.042;.056]** |
| | PT:SM | .472 | **.049** | **.049** | **.049** | **.049** | **.049** | **.049** |
| | | [.457;.488] | **[.043;.056]** | **[.043;.056]** | **[.043;.056]** | **[.043;.056]** | **[.043;.056]** | **[.043;.056]** |
| Ap:As | no PT:SM | .497 | **.052** | **.051** | **.051** | **.051** | **.051** | **.051** |
| | | [.482;.513] | **[.046;.059]** | **[.045;.058]** | **[.045;.058]** | **[.045;.058]** | **[.045;.058]** | **[.045;.058]** |
| | PT:SM | .561 | **.052** | **.051** | **.051** | **.051** | **.051** | **.052** |
| | | [.546;.577] | **[.046;.060]** | **[.045;.059]** | **[.045;.059]** | **[.045;.059]** | **[.045;.059]** | **[.045;.059]** |
| Ap:Am | no PT:SM | .424 | **.051** | **.050** | **.050** | **.050** | **.050** | **.052** |
| | | [.409;.439] | **[.044;.058]** | **[.044;.057]** | **[.044;.057]** | **[.044;.057]** | **[.044;.057]** | **[.046;.060]** |
| | PT:SM | .433 | **.050** | **.050** | **.050** | **.050** | **.050** | **.051** |
| | | [.418;.449] | **[.044;.058]** | **[.043;.057]** | **[.043;.057]** | **[.043;.057]** | **[.043;.057]** | **[.045;.058]** |
| As:Am | no PT:SM | .322 | **.050** | **.050** | **.050** | **.050** | **.050** | .072 |
| | | [.308;.337] | **[.043;.057]** | **[.044;.057]** | **[.044;.057]** | **[.044;.057]** | **[.044;.057]** | [.064;.080] |
| | PT:SM | .337 | **.044** | **.044** | **.044** | **.044** | **.044** | .064 |
| | | [.323;.352] | **[.038;.051]** | **[.038;.051]** | **[.038;.051]** | **[.038;.051]** | **[.038;.051]** | [.056;.072] |
| Ap:As:Am | no PT:SM | .218 | **.052** | **.052** | **.052** | **.052** | **.052** | .115 |
| | | [.206;.231] | **[.046;.059]** | **[.045;.059]** | **[.045;.059]** | **[.045;.059]** | **[.045;.059]** | [.106;.125] |
| | PT:SM | .227 | **.051** | **.050** | **.050** | **.050** | **.050** | .107 |
| | | [.214;.240] | **[.045;.058]** | **[.043;.057]** | **[.044;.058]** | **[.044;.058]** | **[.044;.058]** | [.098;.117] |

Table S6: Type I error rate of the model M1 (see Table 2): The data are simulated using correlated random effects, 18 participants, and 36 stimuli. Represented are the models that do not include random effects associated to the interaction participants:stimuli.

| | | RI | RI-L | MAX | ZCP-sum | ZCP-poly | gANOVA | CS-PCA |
|---|---|---|---|---|---|---|---|---|
| Ap | no PT:SM | .065 | **.051** | **.049** | **.051** | **.051** | **.051** | **.052** |
| | | [.058;.073] | **[.044;.058]** | **[.043;.056]** | **[.045;.059]** | **[.045;.059]** | **[.045;.059]** | **[.045;.059]** |
| | PT:SM | .065 | **.051** | **.051** | **.051** | **.051** | **.051** | **.052** |
| | | [.058;.073] | **[.045;.058]** | **[.044;.059]** | **[.045;.059]** | **[.045;.059]** | **[.045;.059]** | **[.046;.059]** |
| As | no PT:SM | .136 | **.054** | **.052** | **.054** | **.054** | **.054** | **.054** |
| | | [.126;.147] | **[.047;.061]** | **[.045;.059]** | **[.047;.061]** | **[.047;.061]** | **[.047;.061]** | **[.048;.062]** |
| | PT:SM | .136 | **.054** | **.055** | **.053** | **.053** | **.053** | **.054** |
| | | [.125;.147] | **[.047;.061]** | **[.048;.063]** | **[.046;.060]** | **[.046;.060]** | **[.046;.060]** | **[.047;.061]** |
| Am | no PT:SM | .409 | **.047** | *.042* | **.047** | **.047** | **.047** | .373 |
| | | [.394;.425] | **[.041;.054]** | *[.036;.049]* | **[.041;.054]** | **[.041;.054]** | **[.041;.054]** | [.358;.388] |
| | PT:SM | .481 | **.052** | **.051** | **.051** | **.051** | **.051** | .322 |
| | | [.466;.496] | **[.045;.059]** | **[.044;.058]** | **[.045;.059]** | **[.045;.059]** | **[.045;.059]** | [.308;.337] |
| Ap:As | no PT:SM | .534 | **.054** | **.052** | **.054** | **.054** | **.054** | **.054** |
| | | [.519;.549] | **[.048;.062]** | **[.045;.059]** | **[.047;.061]** | **[.047;.061]** | **[.047;.061]** | **[.047;.061]** |
| | PT:SM | .551 | **.052** | **.050** | **.051** | **.051** | **.051** | **.052** |
| | | [.536;.566] | **[.045;.059]** | **[.043;.058]** | **[.044;.058]** | **[.044;.058]** | **[.044;.058]** | **[.045;.059]** |
| Ap:Am | no PT:SM | .377 | **.054** | **.046** | **.054** | **.054** | **.054** | .378 |
| | | [.362;.392] | **[.048;.062]** | **[.040;.053]** | **[.048;.062]** | **[.048;.062]** | **[.048;.062]** | [.363;.393] |
| | PT:SM | .427 | .057 | **.051** | .056 | .056 | .056 | .366 |
| | | [.412;.442] | [.050;.064] | **[.044;.059]** | [.050;.064] | [.050;.064] | [.050;.064] | [.351;.381] |
| As:Am | no PT:SM | .280 | .058 | **.045** | .058 | .058 | .058 | .289 |
| | | [.267;.295] | [.051;.065] | **[.039;.052]** | [.051;.065] | [.051;.065] | [.051;.065] | [.275;.303] |
| | PT:SM | .330 | **.055** | **.050** | **.055** | **.055** | **.055** | .264 |
| | | [.315;.344] | **[.048;.062]** | **[.043;.058]** | **[.048;.062]** | **[.048;.062]** | **[.048;.062]** | [.251;.279] |
| Ap:As:Am | no PT:SM | .174 | **.051** | *.035* | **.051** | **.051** | **.051** | .213 |
| | | [.162;.186] | **[.045;.058]** | *[.029;.041]* | **[.044;.058]** | **[.044;.058]** | **[.044;.058]** | [.200;.226] |
| | PT:SM | .230 | **.053** | **.045** | **.054** | **.054** | **.054** | .286 |
| | | [.217;.243] | **[.047;.061]** | **[.038;.052]** | **[.047;.061]** | **[.047;.061]** | **[.047;.061]** | [.272;.300] |

Table S7: Type I error rate of the model M1 (see Table 2): The data are simulated using correlated random effects, 18 participants, and 36 stimuli. Represented are the models that include random effects associated to the interaction participants:stimuli.

| | | RI+ | RI-L+ | MAX+ | ZCP-sum+ | ZCP-poly+ | gANOVA+ | CS-PCA+ |
|---|---|---|---|---|---|---|---|---|
| Ap | no PT:SM | .065 | **.051** | **.049** | **.052** | **.052** | **.052** | **.052** |
| | | [.058;.073] | **[.045;.058]** | **[.043;.057]** | **[.046;.059]** | **[.046;.059]** | **[.046;.059]** | **[.046;.059]** |
| | PT:SM | .065 | **.051** | **.049** | **.051** | **.051** | **.051** | **.052** |
| | | [.058;.073] | **[.045;.058]** | **[.043;.057]** | **[.045;.059]** | **[.045;.059]** | **[.045;.059]** | **[.046;.059]** |
| As | no PT:SM | .136 | **.055** | **.052** | **.055** | **.055** | **.055** | **.055** |
| | | [.126;.147] | **[.048;.063]** | **[.045;.060]** | **[.048;.062]** | **[.048;.062]** | **[.048;.062]** | **[.048;.062]** |
| | PT:SM | .136 | **.054** | **.054** | **.053** | **.053** | **.053** | **.054** |
| | | [.125;.147] | **[.047;.061]** | **[.047;.062]** | **[.047;.061]** | **[.047;.061]** | **[.047;.061]** | **[.047;.061]** |
| Am | no PT:SM | .450 | *.043* | *.040* | *.043* | *.043* | *.043* | .320 |
| | | [.435;.466] | *[.037;.050]* | *[.034;.047]* | *[.037;.050]* | *[.037;.050]* | *[.037;.050]* | [.306;.335] |
| | PT:SM | .491 | **.051** | **.049** | **.051** | **.051** | **.051** | .312 |
| | | [.476;.506] | **[.045;.059]** | **[.043;.057]** | **[.045;.058]** | **[.045;.058]** | **[.045;.058]** | [.298;.327] |
| Ap:As | no PT:SM | .499 | **.056** | **.052** | **.055** | **.055** | **.055** | **.054** |
| | | [.484;.515] | **[.049;.063]** | **[.045;.059]** | **[.048;.062]** | **[.048;.062]** | **[.048;.062]** | **[.048;.062]** |
| | PT:SM | .540 | **.052** | **.050** | **.051** | **.051** | **.051** | **.052** |
| | | [.525;.556] | **[.045;.059]** | **[.044;.058]** | **[.044;.058]** | **[.044;.058]** | **[.044;.058]** | **[.045;.059]** |
| Ap:Am | no PT:SM | .418 | **.052** | **.047** | **.051** | **.051** | **.051** | .358 |
| | | [.402;.433] | **[.045;.059]** | **[.041;.055]** | **[.045;.059]** | **[.045;.059]** | **[.045;.059]** | [.343;.373] |
| | PT:SM | .438 | .056 | **.050** | **.056** | **.056** | **.056** | .362 |
| | | [.423;.454] | [.050;.064] | **[.044;.058]** | **[.049;.063]** | **[.049;.063]** | **[.049;.063]** | [.348;.378] |
| As:Am | no PT:SM | .331 | **.052** | **.045** | **.052** | **.052** | **.052** | .258 |
| | | [.317;.346] | **[.045;.059]** | **[.038;.052]** | **[.045;.059]** | **[.045;.059]** | **[.045;.059]** | [.245;.272] |
| | PT:SM | .345 | **.054** | **.050** | **.054** | **.054** | **.054** | .257 |
| | | [.331;.360] | **[.047;.061]** | **[.043;.057]** | **[.047;.061]** | **[.047;.061]** | **[.047;.061]** | [.244;.271] |
| Ap:As:Am | no PT:SM | .214 | **.048** | *.038* | **.048** | **.048** | **.048** | .228 |
| | | [.201;.227] | **[.042;.055]** | *[.032;.045]* | **[.042;.055]** | **[.042;.055]** | **[.042;.055]** | [.216;.242] |
| | PT:SM | .242 | **.053** | **.046** | **.053** | **.053** | **.053** | .286 |
| | | [.229;.255] | **[.046;.060]** | **[.040;.054]** | **[.047;.061]** | **[.047;.061]** | **[.047;.061]** | [.272;.300] |

Table S8: Type I error rate of the model M1 (see Table 2): The data are simulated using spherical random effects, 180 participants, and 18 stimuli. The results correspond to the subset of model estimated using the interaction participant:stimuli.

| | | RI+ | RI-L+ | ZCP-poly+ | gANOVA+ |
|---|---|---|---|---|---|
| Ap | no PT:SM | .295 | **.054** | **.053** | **.053** |
| | | [.281;.309] | **[.047;.061]** | **[.047;.061]** | **[.047;.061]** |
| | PT:SM | .302 | **.054** | **.053** | **.053** |
| | | [.288;.316] | **[.047;.061]** | **[.047;.061]** | **[.047;.061]** |
| As | no PT:SM | .056 | **.049** | **.051** | **.051** |
| | | [.050;.064] | **[.043;.056]** | **[.044;.058]** | **[.044;.058]** |
| | PT:SM | .056 | **.049** | **.051** | **.051** |
| | | [.050;.064] | **[.043;.056]** | **[.044;.058]** | **[.044;.058]** |
| Am | no PT:SM | .681 | **.050** | **.048** | **.048** |
| | | [.666;.695] | **[.043;.057]** | **[.042;.055]** | **[.042;.055]** |
| | PT:SM | .692 | **.050** | **.048** | **.048** |
| | | [.677;.706] | **[.043;.057]** | **[.042;.055]** | **[.042;.055]** |
| Ap:As | no PT:SM | .700 | **.055** | **.055** | **.055** |
| | | [.686;.714] | **[.049;.063]** | **[.048;.062]** | **[.048;.062]** |
| | PT:SM | .735 | **.055** | **.055** | **.055** |
| | | [.721;.749] | **[.049;.063]** | **[.048;.062]** | **[.048;.062]** |
| Ap:Am | no PT:SM | .507 | **.052** | **.052** | **.052** |
| | | [.492;.523] | **[.046;.060]** | **[.046;.060]** | **[.046;.060]** |
| | PT:SM | .514 | **.053** | **.053** | **.053** |
| | | [.499;.530] | **[.047;.060]** | **[.046;.060]** | **[.046;.060]** |
| As:Am | no PT:SM | .654 | **.048** | **.048** | **.048** |
| | | [.639;.668] | **[.042;.056]** | **[.042;.056]** | **[.042;.056]** |
| | PT:SM | .662 | **.049** | **.048** | **.048** |
| | | [.648;.677] | **[.042;.056]** | **[.042;.056]** | **[.042;.056]** |
| Ap:As:Am | no PT:SM | .456 | **.052** | **.052** | **.052** |
| | | [.441;.472] | **[.046;.059]** | **[.046;.059]** | **[.046;.059]** |
| | PT:SM | .465 | **.052** | **.052** | **.052** |
| | | [.450;.480] | **[.045;.059]** | **[.045;.059]** | **[.045;.059]** |

Table S9: Type I error rate of the model M1 (see Table 2): The data are simulated using spherical random effects, 180 participants, and 18 stimuli. The results correspond to the subset of model estimated without the interaction participant:stimuli.

| | | RI | RI-L | ZCP-poly | gANOVA |
|---|---|---|---|---|---|
| Ap | no PT:SM | .295 | **.053** | **.053** | **.053** |
| | | [.281;.309] | **[.047;.061]** | **[.046;.060]** | **[.046;.060]** |
| | PT:SM | .302 | **.054** | **.053** | **.053** |
| | | [.288;.316] | **[.047;.061]** | **[.047;.061]** | **[.047;.061]** |
| As | no PT:SM | .056 | **.049** | **.051** | **.051** |
| | | [.050;.064] | **[.043;.056]** | **[.044;.058]** | **[.044;.058]** |
| | PT:SM | .056 | **.049** | **.051** | **.051** |
| | | [.050;.064] | **[.043;.056]** | **[.044;.058]** | **[.044;.058]** |
| Am | no PT:SM | .650 | **.050** | **.049** | **.049** |
| | | [.635;.664] | **[.044;.058]** | **[.043;.056]** | **[.043;.056]** |
| | PT:SM | .683 | **.050** | **.048** | **.048** |
| | | [.669;.698] | **[.043;.057]** | **[.042;.055]** | **[.042;.055]** |
| Ap:As | no PT:SM | .717 | **.054** | **.054** | **.054** |
| | | [.703;.731] | **[.047;.061]** | **[.047;.061]** | **[.047;.061]** |
| | PT:SM | .742 | **.055** | **.055** | **.055** |
| | | [.729;.756] | **[.049;.063]** | **[.048;.062]** | **[.048;.062]** |
| Ap:Am | no PT:SM | .469 | **.055** | **.055** | **.055** |
| | | [.454;.485] | **[.048;.062]** | **[.048;.062]** | **[.048;.062]** |
| | PT:SM | .505 | **.053** | **.053** | **.053** |
| | | [.490;.521] | **[.047;.061]** | **[.047;.061]** | **[.047;.061]** |
| As:Am | no PT:SM | .625 | **.049** | **.049** | **.049** |
| | | [.610;.640] | **[.043;.056]** | **[.043;.056]** | **[.043;.056]** |
| | PT:SM | .655 | **.048** | **.048** | **.048** |
| | | [.640;.670] | **[.042;.056]** | **[.042;.056]** | **[.042;.056]** |
| Ap:As:Am | no PT:SM | .416 | **.054** | **.055** | **.055** |
| | | [.401;.431] | **[.047;.061]** | **[.049;.063]** | **[.049;.063]** |
| | PT:SM | .456 | **.052** | **.052** | **.052** |
| | | [.441;.472] | **[.045;.059]** | **[.045;.059]** | **[.045;.059]** |

Table S10: Type I error rate of the model M1 (see Table 2): The data are simulated using correlated random effects, 180 participants, and 18 stimuli. The results correspond to the subset of model estimated using the interaction participant:stimuli.

| | | RI+ | RI-L+ | ZCP-poly+ | gANOVA+ |
|---|---|---|---|---|---|
| Ap | no PT:SM | .293 | **.054** | **.054** | **.054** |
| | | [.279;.308] | **[.047;.061]** | **[.047;.061]** | **[.047;.061]** |
| | PT:SM | .304 | **.055** | **.054** | **.054** |
| | | [.290;.319] | **[.048;.062]** | **[.048;.062]** | **[.048;.062]** |
| As | no PT:SM | **.055** | **.050** | **.051** | **.051** |
| | | **[.048;.062]** | **[.044;.058]** | **[.045;.059]** | **[.045;.059]** |
| | PT:SM | **.055** | **.049** | **.049** | **.049** |
| | | **[.049;.063]** | **[.043;.056]** | **[.043;.056]** | **[.043;.056]** |
| Am | no PT:SM | .684 | **.054** | **.053** | **.053** |
| | | [.669;.698] | **[.047;.061]** | **[.046;.060]** | **[.046;.060]** |
| | PT:SM | .678 | **.048** | **.048** | **.048** |
| | | [.664;.693] | **[.042;.055]** | **[.042;.055]** | **[.042;.055]** |
| Ap:As | no PT:SM | .688 | .058 | .057 | .057 |
| | | [.674;.703] | [.051;.065] | [.050;.065] | [.050;.065] |
| | PT:SM | .732 | **.053** | **.052** | **.052** |
| | | [.719;.746] | **[.046;.060]** | **[.046;.060]** | **[.046;.060]** |
| Ap:Am | no PT:SM | .505 | **.053** | **.053** | **.053** |
| | | [.490;.521] | **[.047;.061]** | **[.047;.061]** | **[.047;.061]** |
| | PT:SM | .524 | **.051** | **.051** | **.051** |
| | | [.509;.540] | **[.045;.059]** | **[.045;.059]** | **[.045;.059]** |
| As:Am | no PT:SM | .653 | *.042* | *.042* | *.042* |
| | | [.638;.668] | *[.036;.049]* | *[.036;.049]* | *[.036;.049]* |
| | PT:SM | .677 | **.056** | **.056** | **.056** |
| | | [.663;.692] | **[.049;.064]** | **[.049;.063]** | **[.049;.063]** |
| Ap:As:Am | no PT:SM | .443 | **.052** | **.052** | **.052** |
| | | [.428;.459] | **[.045;.059]** | **[.045;.059]** | **[.045;.059]** |
| | PT:SM | .476 | **.055** | **.055** | **.055** |
| | | [.461;.492] | **[.048;.062]** | **[.049;.063]** | **[.049;.063]** |

Table S11: Type I error rate of the model M1 (see Table 2): The data are simulated using correlated random effects, 180 participants, and 18 stimuli. The results correspond to the subset of model estimated without the interaction participant:stimuli.

| | | RI | RI-L | ZCP-poly | gANOVA |
|---|---|---|---|---|---|
| Ap | no PT:SM | .293 | **.053** | **.053** | **.053** |
| | | [.279;.308] | **[.046;.060]** | **[.046;.060]** | **[.046;.060]** |
| | PT:SM | .304 | **.054** | **.054** | **.054** |
| | | [.290;.319] | **[.048;.062]** | **[.048;.062]** | **[.048;.062]** |
| As | no PT:SM | **.055** | **.050** | **.051** | **.051** |
| | | **[.048;.062]** | **[.044;.058]** | **[.045;.059]** | **[.045;.059]** |
| | PT:SM | **.055** | **.049** | **.049** | **.049** |
| | | **[.049;.063]** | **[.043;.056]** | **[.043;.056]** | **[.043;.056]** |
| Am | no PT:SM | .656 | **.054** | **.053** | **.053** |
| | | [.642;.671] | **[.047;.061]** | **[.046;.060]** | **[.046;.060]** |
| | PT:SM | .673 | **.048** | **.048** | **.048** |
| | | [.659;.688] | **[.042;.055]** | **[.042;.055]** | **[.042;.055]** |
| Ap:As | no PT:SM | .714 | .058 | .057 | .057 |
| | | [.700;.728] | [.051;.065] | [.050;.065] | [.050;.065] |
| | PT:SM | .740 | **.053** | **.052** | **.052** |
| | | [.726;.753] | **[.046;.060]** | **[.046;.060]** | **[.046;.060]** |
| Ap:Am | no PT:SM | .468 | **.056** | **.056** | **.056** |
| | | [.452;.483] | **[.049;.063]** | **[.049;.063]** | **[.049;.063]** |
| | PT:SM | .514 | **.051** | **.051** | **.051** |
| | | [.499;.530] | **[.045;.059]** | **[.045;.059]** | **[.045;.059]** |
| As:Am | no PT:SM | .622 | *.043* | *.043* | *.043* |
| | | [.608;.638] | *[.037;.050]* | *[.037;.050]* | *[.037;.050]* |
| | PT:SM | .670 | **.056** | **.056** | **.056** |
| | | [.656;.685] | **[.049;.064]** | **[.049;.063]** | **[.049;.063]** |
| Ap:As:Am | no PT:SM | .404 | **.054** | **.054** | **.054** |
| | | [.389;.419] | **[.047;.061]** | **[.047;.061]** | **[.047;.061]** |
| | PT:SM | .465 | **.055** | **.055** | **.055** |
| | | [.450;.481] | **[.048;.062]** | **[.049;.063]** | **[.049;.063]** |

## 1.2 Design M2

Table S12: Type I error rate of the design M2 (see Table 2): The data are simulated using spherical random effects, 18 participants, and 18 stimuli. Represented are the models that include random effects associated to the interaction participants:stimuli.

| | | RI+ | RI-L+ | MAX+ | ZCP-sum+ | ZCP-poly+ | gANOVA+ | CS-PCA+ |
|---|---|---|---|---|---|---|---|---|
| Ap | no PT:SM | .074 | **.054** | **.056** | **.054** | .056 | **.054** | **.056** |
| | | [.067;.083] | **[.047;.061]** | **[.049;.065]** | **[.047;.061]** | [.050;.064] | **[.048;.062]** | **[.049;.064]** |
| | PT:SM | .075 | **.056** | **.055** | **.053** | **.056** | **.056** | **.056** |
| | | [.067;.084] | **[.049;.063]** | **[.048;.063]** | **[.047;.061]** | **[.049;.063]** | **[.049;.064]** | **[.049;.064]** |
| As | no PT:SM | .086 | **.052** | **.051** | **.052** | **.054** | **.052** | **.053** |
| | | [.078;.096] | **[.046;.060]** | **[.044;.059]** | **[.045;.059]** | **[.047;.061]** | **[.046;.060]** | **[.046;.060]** |
| | PT:SM | .088 | **.053** | **.053** | **.052** | **.053** | **.053** | **.053** |
| | | [.079;.097] | **[.046;.060]** | **[.046;.061]** | **[.045;.059]** | **[.047;.061]** | **[.046;.060]** | **[.046;.060]** |
| Am | no PT:SM | .550 | **.047** | **.047** | .068 | **.050** | **.047** | **.053** |
| | | [.535;.566] | **[.041;.054]** | **[.040;.055]** | [.060;.076] | **[.044;.058]** | **[.041;.054]** | **[.046;.060]** |
| | PT:SM | .560 | **.046** | **.051** | .072 | **.051** | **.046** | **.054** |
| | | [.545;.576] | **[.040;.053]** | **[.044;.058]** | [.064;.080] | **[.045;.058]** | **[.040;.053]** | **[.048;.062]** |
| Ap:As | no PT:SM | .673 | **.048** | **.047** | **.055** | **.055** | **.048** | **.054** |
| | | [.658;.687] | **[.042;.055]** | **[.040;.054]** | **[.048;.063]** | **[.048;.063]** | **[.042;.055]** | **[.048;.062]** |
| | PT:SM | .777 | **.049** | **.056** | **.046** | .060 | **.048** | .060 |
| | | [.764;.790] | **[.043;.056]** | **[.049;.064]** | **[.040;.053]** | [.053;.068] | **[.042;.056]** | [.053;.068] |
| Ap:Am | no PT:SM | .608 | **.048** | *.041* | .069 | .057 | **.048** | .089 |
| | | [.593;.623] | **[.042;.056]** | *[.035;.048]* | [.062;.077] | [.050;.064] | **[.042;.055]** | [.080;.098] |
| | PT:SM | .623 | **.048** | *.041* | .064 | **.056** | **.048** | .079 |
| | | [.608;.638] | **[.042;.055]** | *[.035;.048]* | [.057;.072] | **[.049;.064]** | **[.042;.055]** | [.071;.087] |
| As:Am | no PT:SM | .543 | **.054** | **.043** | .066 | .058 | **.054** | .090 |
| | | [.528;.559] | **[.047;.061]** | **[.037;.051]** | [.059;.074] | [.051;.065] | **[.047;.061]** | [.081;.099] |
| | PT:SM | .560 | **.052** | *.041* | .071 | **.056** | **.052** | .084 |
| | | [.545;.576] | **[.046;.060]** | *[.035;.048]* | [.064;.080] | **[.049;.063]** | **[.046;.060]** | [.076;.093] |
| Ap:As:Am | no PT:SM | .261 | **.052** | *.018* | .074 | .060 | **.052** | .367 |
| | | [.247;.275] | **[.046;.060]** | *[.014;.023]* | [.066;.082] | [.053;.067] | **[.046;.060]** | [.353;.383] |
| | PT:SM | .271 | **.049** | *.024* | .070 | .063 | **.049** | .365 |
| | | [.257;.285] | **[.043;.056]** | *[.019;.029]* | [.062;.078] | [.056;.071] | **[.043;.056]** | [.350;.380] |

Table S13: Estimated type I error rate of the model M2 (see Table 2): The data are simulated using correlated random effects, 18 participants, and 18 stimuli. Represented are the models that do not include random effects associated to the interaction participants:stimuli.

| | | RI | RI-L | MAX | ZCP-sum | ZCP-poly | gANOVA | CS-PCA |
|---|---|---|---|---|---|---|---|---|
| Ap | no PT:SM | .077 | **.051** | **.052** | **.048** | **.053** | **.052** | **.049** |
| | | [.069;.085] | **[.045;.059]** | **[.044;.061]** | **[.042;.055]** | **[.046;.060]** | **[.045;.059]** | **[.043;.056]** |
| | PT:SM | .078 | .057 | **.053** | **.053** | .057 | .057 | **.056** |
| | | [.070;.087] | [.050;.065] | **[.045;.063]** | **[.047;.061]** | [.050;.065] | [.050;.065] | **[.049;.064]** |
| As | no PT:SM | .085 | **.051** | **.050** | **.048** | **.052** | **.051** | **.052** |
| | | [.077;.094] | **[.044;.058]** | **[.043;.059]** | **[.042;.055]** | **[.046;.060]** | **[.044;.058]** | **[.045;.060]** |
| | PT:SM | .086 | **.049** | **.042** | **.048** | **.048** | **.049** | **.049** |
| | | [.078;.096] | **[.043;.056]** | **[.035;.051]** | **[.042;.055]** | **[.042;.055]** | **[.043;.056]** | **[.042;.056]** |
| Am | no PT:SM | .443 | **.056** | *.042* | .072 | .060 | **.056** | **.056** |
| | | [.428;.459] | **[.049;.064]** | *[.035;.050]* | [.064;.080] | [.053;.068] | **[.049;.064]** | **[.049;.064]** |
| | PT:SM | .535 | **.053** | **.050** | .068 | .059 | **.053** | **.056** |
| | | [.520;.550] | **[.046;.060]** | **[.042;.060]** | [.061;.077] | [.052;.067] | **[.046;.060]** | **[.049;.064]** |
| Ap:As | no PT:SM | .816 | *.041* | *.036* | *.038* | **.046** | *.041* | *.042* |
| | | [.804;.828] | *[.035;.047]* | *[.029;.043]* | *[.033;.045]* | **[.040;.053]** | *[.035;.047]* | *[.036;.049]* |
| | PT:SM | .832 | **.051** | **.046** | **.050** | .061 | **.051** | **.051** |
| | | [.820;.844] | **[.045;.059]** | **[.038;.055]** | **[.044;.057]** | [.054;.069] | **[.045;.058]** | **[.044;.058]** |
| Ap:Am | no PT:SM | .472 | **.055** | *.032* | .069 | .056 | **.055** | .079 |
| | | [.457;.487] | **[.049;.063]** | *[.026;.039]* | [.062;.078] | [.050;.064] | **[.049;.063]** | [.071;.088] |
| | PT:SM | .552 | **.053** | *.040* | .066 | .057 | **.052** | .079 |
| | | [.537;.568] | **[.046;.060]** | *[.033;.049]* | [.059;.074] | [.050;.064] | **[.046;.060]** | [.071;.088] |
| As:Am | no PT:SM | .411 | .060 | *.037* | .084 | .066 | .060 | .089 |
| | | [.396;.426] | [.053;.068] | *[.031;.045]* | [.076;.093] | [.059;.074] | [.053;.068] | [.080;.098] |
| | PT:SM | .496 | **.050** | **.045** | .074 | .060 | **.051** | .084 |
| | | [.481;.512] | **[.044;.058]** | **[.037;.054]** | [.066;.082] | [.053;.068] | **[.045;.058]** | [.076;.094] |
| Ap:As:Am | no PT:SM | .113 | .082 | *.009* | .084 | .068 | .082 | .304 |
| | | [.104;.123] | [.074;.091] | *[.006;.014]* | [.076;.093] | [.061;.077] | [.074;.091] | [.289;.319] |
| | PT:SM | .190 | .058 | *.015* | .085 | .062 | .058 | .451 |
| | | [.178;.203] | [.052;.066] | *[.011;.020]* | [.077;.094] | [.054;.069] | [.052;.066] | [.435;.468] |

Table S14: Type I error rate of the model M2 (see Table 2): The data are simulated using correlated random effects, 18 participants, and 18 stimuli. Represented are the models that include random effects associated to the interaction participants:stimuli.

| | | RI+ | RI-L+ | MAX+ | ZCP-sum+ | ZCP-poly+ | gANOVA+ | CS-PCA+ |
|---|---|---|---|---|---|---|---|---|
| Ap | no PT:SM | .077 | **.054** | **.045** | **.052** | **.055** | **.054** | **.051** |
| | | [.069;.085] | **[.047;.061]** | **[.038;.054]** | **[.045;.059]** | **[.048;.062]** | **[.047;.061]** | **[.045;.059]** |
| | PT:SM | .078 | .058 | **.053** | **.053** | .057 | .057 | **.056** |
| | | [.070;.087] | [.051;.065] | **[.045;.062]** | **[.047;.061]** | [.050;.065] | [.050;.065] | **[.049;.064]** |
| As | no PT:SM | .085 | **.054** | **.051** | **.051** | **.055** | **.054** | **.053** |
| | | [.077;.094] | **[.047;.061]** | **[.043;.060]** | **[.045;.059]** | **[.048;.063]** | **[.047;.061]** | **[.046;.060]** |
| | PT:SM | .086 | **.049** | **.044** | **.048** | **.048** | **.049** | **.046** |
| | | [.078;.096] | **[.043;.056]** | **[.036;.052]** | **[.042;.055]** | **[.042;.055]** | **[.043;.056]** | **[.040;.054]** |
| Am | no PT:SM | .537 | **.051** | **.048** | .066 | **.054** | **.051** | **.053** |
| | | [.522;.553] | **[.045;.059]** | **[.040;.057]** | [.059;.075] | **[.048;.062]** | **[.045;.058]** | **[.046;.060]** |
| | PT:SM | .580 | **.053** | **.054** | .068 | .059 | **.052** | **.055** |
| | | [.565;.596] | **[.046;.060]** | **[.046;.064]** | [.061;.077] | [.052;.067] | **[.046;.060]** | **[.048;.063]** |
| Ap:As | no PT:SM | .671 | **.046** | *.033* | **.051** | **.054** | **.046** | *.042* |
| | | [.657;.686] | **[.040;.053]** | *[.027;.041]* | **[.045;.058]** | **[.047;.061]** | **[.040;.053]** | *[.036;.050]* |
| | PT:SM | .762 | **.052** | **.049** | **.051** | .061 | **.052** | **.050** |
| | | [.749;.776] | **[.045;.059]** | **[.041;.058]** | **[.045;.058]** | [.054;.069] | **[.045;.059]** | **[.043;.058]** |
| Ap:Am | no PT:SM | .596 | **.046** | *.036* | .066 | **.051** | **.046** | .075 |
| | | [.581;.612] | **[.040;.053]** | *[.030;.044]* | [.059;.075] | **[.045;.059]** | **[.040;.053]** | [.067;.084] |
| | PT:SM | .607 | **.053** | **.044** | .065 | .056 | **.052** | .079 |
| | | [.592;.622] | **[.046;.060]** | **[.036;.052]** | [.058;.073] | [.050;.064] | **[.046;.060]** | [.070;.088] |
| As:Am | no PT:SM | .543 | **.052** | *.041* | .078 | .059 | **.052** | .089 |
| | | [.528;.559] | **[.045;.059]** | *[.034;.049]* | [.070;.086] | [.052;.067] | **[.046;.059]** | [.081;.099] |
| | PT:SM | .568 | **.050** | **.045** | .073 | .060 | **.050** | .086 |
| | | [.553;.584] | **[.044;.057]** | **[.037;.053]** | [.065;.081] | [.053;.068] | **[.044;.058]** | [.077;.095] |
| Ap:As:Am | no PT:SM | .257 | **.054** | *.013* | .080 | .057 | **.054** | .402 |
| | | [.244;.271] | **[.047;.061]** | *[.009;.018]* | [.072;.089] | [.050;.064] | **[.048;.062]** | [.386;.418] |
| | PT:SM | .272 | .057 | *.015* | .083 | .061 | .057 | .452 |
| | | [.258;.286] | [.050;.065] | *[.011;.020]* | [.075;.092] | [.054;.069] | [.050;.065] | [.436;.468] |

Table S15: Type I error rate of the model M2 (see Table 2): The data are simulated using spherical random effects, 18 participants, and 36 stimuli. Represented are the models that include random effects associated to the interaction participants:stimuli.

| | | RI | RI-L | MAX | ZCP-sum | ZCP-poly | gANOVA | CS-PCA |
|---|---|---|---|---|---|---|---|---|
| Ap | no PT:SM | .062 | **.054** | **.054** | **.051** | **.054** | **.054** | **.055** |
| | | [.055;.070] | **[.047;.061]** | **[.047;.063]** | **[.044;.058]** | **[.048;.062]** | **[.047;.061]** | **[.048;.062]** |
| | PT:SM | .062 | **.054** | **.054** | **.052** | **.054** | **.054** | **.054** |
| | | [.055;.070] | **[.047;.061]** | **[.047;.062]** | **[.046;.059]** | **[.048;.062]** | **[.048;.062]** | **[.047;.061]** |
| As | no PT:SM | .136 | **.051** | **.051** | **.049** | **.052** | **.050** | **.052** |
| | | [.126;.148] | **[.044;.058]** | **[.044;.059]** | **[.043;.056]** | **[.045;.059]** | **[.044;.058]** | **[.045;.059]** |
| | PT:SM | .139 | **.054** | .059 | **.053** | .058 | **.054** | .058 |
| | | [.129;.150] | **[.047;.061]** | [.052;.068] | **[.046;.060]** | [.051;.065] | **[.047;.061]** | [.051;.066] |
| Am | no PT:SM | .584 | **.054** | **.053** | .069 | **.056** | **.053** | **.056** |
| | | [.569;.599] | **[.047;.061]** | **[.046;.061]** | [.062;.077] | **[.049;.063]** | **[.047;.061]** | **[.049;.064]** |
| | PT:SM | .633 | **.051** | **.053** | .066 | .056 | **.051** | .057 |
| | | [.618;.648] | **[.045;.058]** | **[.046;.061]** | [.059;.075] | [.050;.064] | **[.044;.058]** | [.050;.065] |
| Ap:As | no PT:SM | .906 | *.041* | **.044** | *.043* | **.046** | *.041* | **.046** |
| | | [.896;.915] | *[.036;.048]* | **[.038;.051]** | *[.037;.049]* | **[.040;.053]** | *[.036;.048]* | **[.040;.053]** |
| | PT:SM | .926 | **.046** | **.052** | **.046** | **.052** | **.046** | **.053** |
| | | [.918;.934] | **[.040;.053]** | **[.045;.060]** | **[.040;.053]** | **[.045;.059]** | **[.040;.053]** | **[.046;.061]** |
| Ap:Am | no PT:SM | .723 | .059 | .065 | .077 | .069 | .058 | .077 |
| | | [.709;.737] | [.052;.066] | [.057;.074] | [.069;.086] | [.061;.077] | [.051;.066] | [.069;.085] |
| | PT:SM | .782 | **.054** | .059 | .072 | .064 | **.054** | .066 |
| | | [.769;.795] | **[.048;.062]** | [.052;.068] | [.064;.081] | [.057;.072] | **[.048;.062]** | [.059;.074] |
| As:Am | no PT:SM | .478 | .061 | **.056** | .092 | .069 | .061 | .122 |
| | | [.463;.493] | [.054;.069] | **[.049;.065]** | [.083;.101] | [.062;.077] | [.054;.069] | [.112;.133] |
| | PT:SM | .565 | **.051** | **.054** | .081 | .057 | **.051** | .081 |
| | | [.550;.581] | **[.045;.059]** | **[.047;.062]** | [.073;.089] | [.050;.065] | **[.045;.059]** | [.073;.090] |
| Ap:As:Am | no PT:SM | .250 | .075 | *.036* | .103 | .087 | .075 | .409 |
| | | [.237;.264] | [.067;.083] | *[.030;.043]* | [.094;.112] | [.079;.096] | [.067;.083] | [.394;.425] |
| | PT:SM | .360 | **.049** | *.039* | .085 | .060 | **.049** | .195 |
| | | [.345;.375] | **[.043;.056]** | *[.033;.046]* | [.077;.094] | [.053;.068] | **[.043;.056]** | [.183;.208] |

Table S16: Type I error rate of the model M2 (see Table 2): The data are simulated using spherical random effects, 18 participants, and 36 stimuli. Represented are the models that include random effects associated to the interaction participants:stimuli.

| | | RI+ | RI-L+ | MAX+ | ZCP-sum+ | ZCP-poly+ | gANOVA+ | CS-PCA+ |
|---|---|---|---|---|---|---|---|---|
| Ap | no PT:SM | .062 | **.054** | **.051** | **.053** | **.055** | **.054** | **.055** |
| | | [.055;.070] | **[.048;.062]** | **[.044;.059]** | **[.046;.060]** | **[.049;.063]** | **[.048;.062]** | **[.048;.062]** |
| | PT:SM | .062 | **.054** | **.055** | **.053** | **.054** | **.055** | **.053** |
| | | [.055;.070] | **[.048;.062]** | **[.048;.063]** | **[.046;.060]** | **[.048;.062]** | **[.048;.062]** | **[.047;.061]** |
| As | no PT:SM | .136 | **.053** | **.053** | **.053** | **.054** | **.053** | **.055** |
| | | [.126;.148] | **[.047;.061]** | **[.046;.061]** | **[.046;.060]** | **[.048;.062]** | **[.047;.061]** | **[.048;.062]** |
| | PT:SM | .139 | **.054** | .059 | **.053** | .058 | **.054** | .058 |
| | | [.129;.150] | **[.047;.061]** | [.051;.067] | **[.047;.060]** | [.051;.065] | **[.047;.061]** | [.051;.066] |
| Am | no PT:SM | .660 | **.051** | **.052** | .066 | **.051** | **.050** | **.052** |
| | | [.645;.674] | **[.044;.058]** | **[.045;.061]** | [.058;.074] | **[.044;.058]** | **[.044;.058]** | **[.045;.059]** |
| | PT:SM | .666 | **.051** | **.053** | .066 | **.056** | **.050** | .057 |
| | | [.652;.681] | **[.044;.058]** | **[.046;.061]** | [.059;.074] | **[.049;.064]** | **[.044;.057]** | [.050;.065] |
| Ap:As | no PT:SM | .817 | **.047** | **.046** | **.052** | **.051** | **.047** | **.052** |
| | | [.805;.829] | **[.041;.054]** | **[.040;.054]** | **[.046;.060]** | **[.045;.058]** | **[.041;.054]** | **[.045;.059]** |
| | PT:SM | .885 | **.047** | **.053** | **.047** | **.052** | **.047** | **.053** |
| | | [.875;.895] | **[.041;.054]** | **[.046;.061]** | **[.040;.054]** | **[.046;.059]** | **[.041;.054]** | **[.046;.061]** |
| Ap:Am | no PT:SM | .809 | **.055** | .064 | .075 | .063 | **.054** | .068 |
| | | [.797;.821] | **[.048;.062]** | [.056;.073] | [.067;.083] | [.056;.071] | **[.048;.062]** | [.060;.076] |
| | PT:SM | .824 | **.054** | .059 | .072 | .064 | **.054** | .067 |
| | | [.812;.836] | **[.048;.062]** | [.052;.068] | [.064;.080] | [.057;.072] | **[.048;.062]** | [.060;.076] |
| As:Am | no PT:SM | .606 | **.051** | **.053** | .081 | .058 | **.051** | .086 |
| | | [.591;.621] | **[.045;.059]** | **[.045;.061]** | [.073;.090] | [.051;.065] | **[.045;.059]** | [.077;.095] |
| | PT:SM | .622 | **.051** | **.051** | .081 | .057 | **.051** | .080 |
| | | [.607;.637] | **[.045;.058]** | **[.045;.059]** | [.073;.089] | [.050;.065] | **[.045;.058]** | [.072;.089] |
| Ap:As:Am | no PT:SM | .446 | **.051** | *.040* | .092 | .070 | **.051** | .249 |
| | | [.431;.462] | **[.045;.059]** | *[.034;.047]* | [.083;.101] | [.063;.079] | **[.045;.059]** | [.235;.263] |
| | PT:SM | .463 | **.049** | *.040* | .085 | .059 | **.049** | .189 |
| | | [.448;.479] | **[.042;.056]** | *[.034;.047]* | [.076;.094] | [.052;.067] | **[.042;.056]** | [.177;.202] |

Table S17: Type I error rate of the model M2 (see Table 2): The data are simulated using correlated random effects, 18 participants, and 36 stimuli. Represented are the models that do not include random effects associated to the interaction participants:stimuli.

| | | RI | RI-L | MAX | ZCP-sum | ZCP-poly | gANOVA | CS-PCA |
|---|---|---|---|---|---|---|---|---|
| Ap | no PT:SM | .058 | **.048** | **.050** | **.047** | **.048** | **.048** | **.049** |
| | | [.051;.065] | **[.042;.055]** | **[.043;.059]** | **[.041;.054]** | **[.042;.055]** | **[.042;.055]** | **[.043;.057]** |
| | PT:SM | .059 | **.047** | **.050** | **.047** | **.047** | **.047** | **.050** |
| | | [.052;.067] | **[.041;.054]** | **[.042;.060]** | **[.041;.054]** | **[.041;.054]** | **[.041;.054]** | **[.043;.058]** |
| As | no PT:SM | .134 | **.050** | **.056** | **.046** | **.050** | **.050** | **.050** |
| | | [.124;.145] | **[.044;.058]** | **[.048;.065]** | **[.040;.053]** | **[.043;.057]** | **[.044;.058]** | **[.043;.057]** |
| | PT:SM | .140 | **.050** | **.055** | **.044** | **.053** | **.050** | **.056** |
| | | [.129;.151] | **[.044;.058]** | **[.047;.065]** | **[.039;.051]** | **[.046;.060]** | **[.044;.058]** | **[.049;.065]** |
| Am | no PT:SM | .564 | **.050** | **.045** | .060 | **.052** | **.050** | **.050** |
| | | [.549;.580] | **[.044;.057]** | **[.038;.054]** | [.053;.068] | **[.046;.060]** | **[.044;.057]** | **[.044;.058]** |
| | PT:SM | .635 | **.048** | **.050** | .066 | **.053** | **.048** | **.053** |
| | | [.621;.650] | **[.041;.055]** | **[.042;.060]** | [.058;.074] | **[.046;.060]** | **[.041;.055]** | **[.046;.061]** |
| Ap:As | no PT:SM | .908 | **.044** | **.048** | **.046** | **.049** | **.044** | **.045** |
| | | [.899;.917] | **[.039;.051]** | **[.041;.057]** | **[.040;.053]** | **[.043;.056]** | **[.039;.051]** | **[.039;.053]** |
| | PT:SM | .923 | **.051** | **.052** | **.052** | .056 | **.051** | **.053** |
| | | [.915;.932] | **[.044;.058]** | **[.044;.062]** | **[.046;.060]** | [.050;.064] | **[.044;.058]** | **[.046;.061]** |
| Ap:Am | no PT:SM | .698 | .059 | **.055** | .075 | .067 | .059 | .077 |
| | | [.684;.712] | [.052;.067] | **[.047;.064]** | [.068;.084] | [.060;.075] | [.052;.067] | [.068;.086] |
| | PT:SM | .770 | **.054** | **.058** | .070 | .064 | **.054** | .073 |
| | | [.757;.783] | **[.048;.062]** | **[.049;.068]** | [.062;.078] | [.057;.072] | **[.048;.062]** | [.065;.083] |
| As:Am | no PT:SM | .478 | **.053** | *.037* | .094 | .063 | **.053** | .118 |
| | | [.463;.494] | **[.046;.060]** | *[.030;.044]* | [.086;.104] | [.056;.071] | **[.046;.060]** | [.108;.128] |
| | PT:SM | .540 | **.045** | *.034* | .080 | **.051** | **.045** | .117 |
| | | [.525;.556] | **[.039;.052]** | *[.028;.043]* | [.072;.089] | **[.044;.058]** | **[.039;.052]** | [.107;.129] |
| Ap:As:Am | no PT:SM | .245 | .083 | *.026* | .113 | .086 | .083 | .457 |
| | | [.232;.259] | [.075;.092] | *[.020;.032]* | [.104;.124] | [.078;.096] | [.075;.092] | [.441;.473] |
| | PT:SM | .351 | .058 | *.028* | .106 | .068 | .058 | .502 |
| | | [.337;.366] | [.051;.065] | *[.022;.036]* | [.097;.116] | [.061;.077] | [.051;.065] | [.485;.519] |

Table S18: Type I error rate of the model M2 (see Table 2): The data are simulated using correlated random effects, 18 participants, and 36 stimuli. Represented are the models that include random effects associated to the interaction participants:stimuli.

| | | RI+ | RI-L+ | MAX+ | ZCP-sum+ | ZCP-poly+ | gANOVA+ | CS-PCA+ |
|---|---|---|---|---|---|---|---|---|
| Ap | no PT:SM | .058 | **.049** | **.048** | **.048** | **.049** | **.048** | **.050** |
| | | [.051;.065] | **[.043;.056]** | **[.040;.057]** | **[.042;.056]** | **[.043;.056]** | **[.042;.056]** | **[.043;.057]** |
| | PT:SM | .059 | **.047** | **.049** | **.047** | **.047** | **.047** | **.048** |
| | | [.052;.067] | **[.041;.054]** | **[.041;.058]** | **[.041;.054]** | **[.041;.054]** | **[.041;.054]** | **[.042;.056]** |
| As | no PT:SM | .134 | **.052** | **.050** | **.048** | **.052** | **.052** | **.052** |
| | | [.124;.145] | **[.046;.060]** | **[.042;.060]** | **[.042;.055]** | **[.046;.060]** | **[.046;.060]** | **[.045;.060]** |
| | PT:SM | .140 | **.051** | **.051** | **.045** | **.053** | **.050** | .057 |
| | | [.129;.151] | **[.044;.058]** | **[.043;.060]** | **[.039;.052]** | **[.046;.060]** | **[.044;.058]** | [.050;.066] |
| Am | no PT:SM | .642 | **.046** | *.040* | **.055** | **.050** | **.046** | **.048** |
| | | [.627;.657] | **[.040;.053]** | *[.033;.049]* | **[.048;.063]** | **[.043;.057]** | **[.040;.053]** | **[.041;.056]** |
| | PT:SM | .672 | **.047** | **.052** | .066 | **.053** | **.047** | **.054** |
| | | [.658;.687] | **[.041;.054]** | **[.044;.061]** | [.058;.074] | **[.046;.060]** | **[.041;.054]** | **[.047;.062]** |
| Ap:As | no PT:SM | .813 | **.049** | **.046** | **.053** | **.055** | **.049** | **.044** |
| | | [.801;.825] | **[.043;.056]** | **[.038;.056]** | **[.046;.060]** | **[.048;.062]** | **[.043;.056]** | **[.038;.052]** |
| | PT:SM | .881 | **.051** | **.050** | **.052** | .057 | **.051** | **.050** |
| | | [.871;.891] | **[.045;.058]** | **[.042;.059]** | **[.046;.060]** | [.050;.064] | **[.045;.058]** | **[.044;.058]** |
| Ap:Am | no PT:SM | .794 | **.053** | **.053** | .072 | .063 | **.053** | .075 |
| | | [.781;.806] | **[.047;.061]** | **[.044;.062]** | [.064;.080] | [.056;.071] | **[.047;.061]** | [.067;.084] |
| | PT:SM | .809 | **.054** | **.058** | .069 | .064 | **.054** | .073 |
| | | [.797;.821] | **[.047;.061]** | **[.049;.067]** | [.062;.078] | [.056;.072] | **[.047;.061]** | [.065;.083] |
| As:Am | no PT:SM | .610 | *.042* | *.036* | .082 | **.050** | *.042* | .113 |
| | | [.595;.625] | *[.036;.049]* | *[.029;.044]* | [.073;.090] | **[.044;.058]** | *[.036;.049]* | [.103;.124] |
| | PT:SM | .609 | **.045** | *.035* | .080 | **.051** | **.045** | .116 |
| | | [.594;.625] | **[.039;.052]** | *[.029;.043]* | [.072;.089] | **[.044;.058]** | **[.039;.052]** | [.106;.127] |
| Ap:As:Am | no PT:SM | .420 | .060 | *.028* | .103 | .069 | .060 | .494 |
| | | [.405;.436] | [.053;.068] | *[.022;.035]* | [.094;.113] | [.062;.077] | [.053;.068] | [.478;.511] |
| | PT:SM | .448 | .057 | *.027* | .106 | .067 | .056 | .493 |
| | | [.433;.463] | [.050;.064] | *[.022;.034]* | [.097;.116] | [.059;.075] | [.050;.064] | [.477;.510] |

## 1.3 Design M4

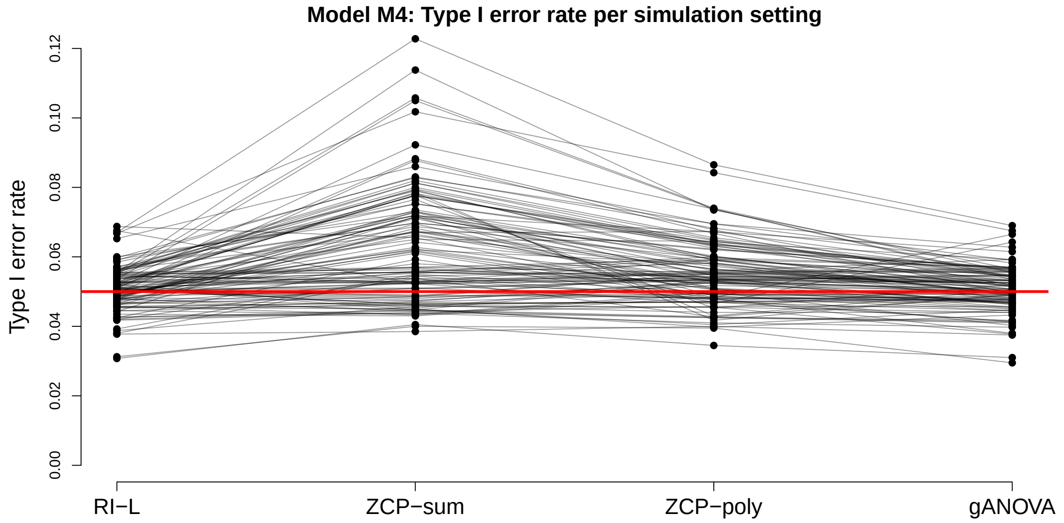


Figure S1: Type I error rate of the model M4 for all simulations setting (1 sample sizes × 2 correlations of random effects × 2 interactions in simulation × 2 interactions in estimation × 15 effects = 120 settings ). The spherical correlation structures (RI-L and gANOVA) produce results closer to the nominal level.

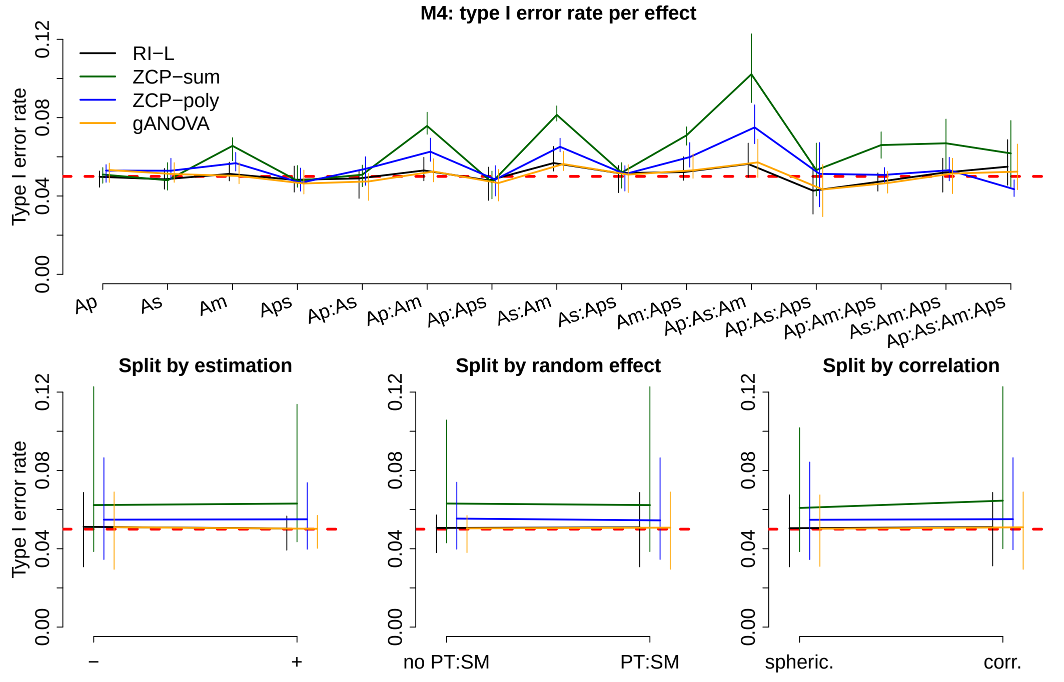


Figure S2: Type I error rate of the model M4 split given the simulations settings. The vertical lines indicate the range of all simulations within the condition. No simulation setting tend to have an effect on the type I error rate. The factor $A_M$ and its interaction have also a higher deviation from the nominal level.

Table S19: Type I error rate of the model M4 (see Table 2): The data are simulated using spherical random effects, 18 participants, and 18 stimuli. Represented are the models that do not include random effects associated to the interaction participants:stimuli.

| | | RI | RI-L | ZCP-sum | ZCP-poly | gANOVA |
|---|---|---|---|---|---|---|
| Ap | no PT:SM | .078 [.070;.087] | **.050 [.043;.057]** | **.052 [.046;.060]** | **.054 [.047;.061]** | **.055 [.048;.062]** |
| | PT:SM | .080 [.072;.089] | **.053 [.046;.060]** | **.052 [.046;.060]** | **.055 [.049;.063]** | .056 [.050;.064] |
| As | no PT:SM | .091 [.082;.100] | **.046 [.040;.053]** | *.043* [.037;.050] | **.049 [.043;.056]** | **.048 [.042;.055]** |
| | PT:SM | .094 [.086;.104] | *.044* [.038;.050] | *.043* [.037;.050] | **.048 [.042;.056]** | **.047 [.041;.054]** |
| Am | no PT:SM | .507 [.492;.523] | **.052 [.045;.059]** | .067 [.060;.075] | .056 [.050;.064] | **.051 [.044;.058]** |
| | PT:SM | .540 [.525;.555] | **.049 [.043;.056]** | .067 [.060;.075] | **.053 [.046;.060]** | **.047 [.041;.054]** |
| Aps | no PT:SM | .417 [.402;.433] | **.051 [.044;.058]** | **.049 [.043;.056]** | **.048 [.042;.055]** | **.048 [.042;.055]** |
| | PT:SM | .422 [.407;.438] | **.051 [.045;.058]** | **.046 [.040;.053]** | **.047 [.041;.054]** | **.048 [.042;.055]** |
| Ap:As | no PT:SM | .789 [.776;.802] | *.039* [.033;.045] | **.046 [.040;.053]** | **.046 [.039;.052]** | *.038* [.032;.044] |
| | PT:SM | .820 [.808;.832] | **.053 [.046;.060]** | **.056 [.049;.063]** | .059 [.052;.067] | **.051 [.044;.058]** |
| Ap:Am | no PT:SM | .545 [.530;.561] | .060 [.053;.068] | .083 [.075;.092] | .070 [.062;.078] | .059 [.052;.067] |
| | PT:SM | .582 [.566;.597] | **.053 [.046;.060]** | .078 [.070;.087] | .064 [.057;.072] | **.052 [.046;.059]** |
| Ap:Aps | no PT:SM | .502 [.487;.518] | *.038* [.032;.044] | *.039* [.033;.045] | *.040* [.034;.047] | *.038* [.032;.044] |
| | PT:SM | .519 [.504;.535] | **.055 [.048;.062]** | **.053 [.046;.060]** | **.054 [.047;.061]** | **.053 [.046;.060]** |
| As:Am | no PT:SM | .498 [.482;.513] | .059 [.052;.067] | .083 [.075;.092] | .068 [.061;.077] | .058 [.051;.066] |
| | PT:SM | .545 [.530;.560] | **.056 [.049;.063]** | .080 [.072;.089] | .064 [.056;.072] | **.056 [.049;.063]** |
| As:Aps | no PT:SM | .456 [.441;.471] | *.042* [.036;.048] | **.044 [.038;.051]** | *.042* [.037;.049] | *.042* [.036;.048] |
| | PT:SM | .476 [.461;.492] | **.054 [.047;.061]** | **.052 [.046;.060]** | **.054 [.047;.061]** | **.052 [.045;.059]** |
| Am:Aps | no PT:SM | .162 [.151;.174] | .060 [.053;.068] | .072 [.064;.080] | .067 [.060;.075] | .062 [.054;.069] |
| | PT:SM | .190 [.178;.203] | **.048 [.042;.055]** | .074 [.066;.082] | .060 [.053;.068] | **.050 [.044;.057]** |
| Ap:As:Am | no PT:SM | .190 [.179;.203] | .067 [.059;.075] | .102 [.093;.112] | .084 [.076;.093] | .068 [.060;.076] |
| | PT:SM | .264 [.251;.279] | **.051 [.045;.058]** | .088 [.080;.097] | .068 [.060;.076] | **.052 [.045;.059]** |
| Ap:As:Aps | no PT:SM | .378 [.364;.394] | *.031* [.026;.037] | *.041* [.035;.047] | *.034* [.029;.041] | *.031* [.026;.037] |
| | PT:SM | .385 [.370;.401] | **.054 [.047;.061]** | .065 [.058;.073] | .064 [.057;.073] | **.054 [.048;.062]** |
| Ap:Am:Aps | no PT:SM | .104 [.095;.114] | **.050 [.043;.057]** | .062 [.055;.070] | **.050 [.044;.058]** | **.049 [.043;.056]** |
| | PT:SM | .156 [.145;.167] | **.049 [.043;.056]** | .063 [.056;.071] | **.053 [.046;.060]** | **.047 [.041;.054]** |
| As:Am:Aps | no PT:SM | .104 [.095;.114] | **.055 [.048;.062]** | .057 [.050;.064] | **.052 [.046;.060]** | **.053 [.047;.061]** |
| | PT:SM | .148 [.137;.159] | **.049 [.043;.056]** | .062 [.054;.069] | **.049 [.043;.056]** | **.049 [.043;.056]** |
| Ap:As:Am:Aps | no PT:SM | *.038* [.032;.044] | .068 [.060;.076] | **.052 [.046;.060]** | **.046 [.040;.054]** | .064 [.057;.072] |
| | PT:SM | **.055 [.048;.063]** | **.047 [.041;.054]** | **.045 [.039;.052]** | *.040* [.035;.047] | **.045 [.039;.052]** |

Table S20: Type I error rate of the model M4 (see Table 2): The data are simulated using sphercial random effect, 18 participants, and 18 stimuli. Represented are the models that include random effects associated to the interaction participants:stimuli.

| | | RI+ | RI-L+ | ZCP-sum+ | ZCP-poly+ | gANOVA+ |
|---|---|---|---|---|---|---|
| Ap | no PT:SM | .079 [.071;.088] | **.052 [.045;.059]** | **.054 [.048;.062]** | **.056 [.049;.064]** | **.056 [.049;.063]** |
| | PT:SM | .081 [.073;.090] | **.053 [.046;.060]** | **.053 [.046;.060]** | **.056 [.049;.063]** | .057 [.050;.064] |
| As | no PT:SM | .091 [.083;.100] | **.048 [.042;.055]** | **.047 [.041;.054]** | **.053 [.046;.060]** | **.050 [.044;.058]** |
| | PT:SM | .094 [.086;.104] | **.044 [.039;.051]** | *.044* [.038;.050] | **.050 [.043;.057]** | **.047 [.041;.054]** |
| Am | no PT:SM | .594 [.578;.609] | **.049 [.043;.056]** | .064 [.057;.072] | **.056 [.049;.063]** | **.048 [.042;.055]** |
| | PT:SM | .601 [.586;.617] | **.048 [.042;.056]** | .066 [.059;.075] | **.053 [.046;.060]** | **.046 [.040;.054]** |
| Aps | no PT:SM | .311 [.297;.326] | **.055 [.049;.063]** | **.056 [.049;.063]** | **.054 [.048;.062]** | **.053 [.047;.061]** |
| | PT:SM | .350 [.336;.366] | **.051 [.044;.058]** | **.046 [.040;.053]** | **.047 [.041;.054]** | **.048 [.041;.055]** |
| Ap:As | no PT:SM | .624 [.609;.639] | **.047 [.041;.054]** | **.056 [.049;.063]** | **.052 [.046;.060]** | **.046 [.039;.052]** |
| | PT:SM | .702 [.688;.717] | **.053 [.046;.060]** | **.056 [.049;.063]** | .060 [.053;.068] | **.052 [.045;.059]** |
| Ap:Am | no PT:SM | .678 [.664;.693] | **.056 [.049;.063]** | .078 [.070;.086] | .065 [.058;.073] | **.055 [.048;.062]** |
| | PT:SM | .663 [.648;.678] | **.052 [.046;.060]** | .078 [.070;.087] | .063 [.056;.071] | **.052 [.045;.059]** |
| Ap:Aps | no PT:SM | .350 [.336;.365] | **.046 [.040;.053]** | **.047 [.041;.054]** | **.047 [.041;.054]** | **.044 [.039;.051]** |
| | PT:SM | .402 [.387;.417] | **.055 [.048;.062]** | **.052 [.046;.060]** | **.056 [.049;.063]** | **.054 [.047;.061]** |
| As:Am | no PT:SM | .641 [.626;.656] | **.053 [.046;.060]** | .078 [.070;.087] | .062 [.055;.070] | **.053 [.046;.060]** |
| | PT:SM | .638 [.623;.653] | **.054 [.048;.062]** | .080 [.072;.088] | .063 [.056;.071] | **.054 [.048;.062]** |
| As:Aps | no PT:SM | .292 [.278;.306] | **.050 [.043;.057]** | **.052 [.046;.060]** | **.049 [.043;.056]** | **.050 [.043;.057]** |
| | PT:SM | .348 [.334;.363] | **.054 [.048;.062]** | **.054 [.047;.061]** | **.054 [.047;.061]** | **.052 [.046;.060]** |
| Am:Aps | no PT:SM | .264 [.250;.278] | **.054 [.047;.061]** | .069 [.061;.077] | .060 [.053;.067] | **.054 [.047;.061]** |
| | PT:SM | .248 [.234;.261] | **.048 [.042;.055]** | .073 [.065;.082] | .059 [.052;.067] | **.049 [.043;.056]** |
| Ap:As:Am | no PT:SM | .390 [.375;.406] | **.052 [.046;.060]** | .092 [.084;.102] | .074 [.066;.082] | **.054 [.047;.061]** |
| | PT:SM | .411 [.396;.426] | **.050 [.043;.057]** | .088 [.079;.097] | .067 [.059;.075] | **.050 [.043;.057]** |
| Ap:As:Aps | no PT:SM | .168 [.157;.181] | **.046 [.040;.053]** | **.051 [.045;.058]** | **.048 [.042;.055]** | **.049 [.043;.056]** |
| | PT:SM | .216 [.203;.229] | .056 [.050;.064] | .067 [.060;.075] | .067 [.060;.075] | **.056 [.049;.064]** |
| Ap:Am:Aps | no PT:SM | .216 [.204;.230] | *.042* [.037;.049] | .059 [.052;.067] | **.047 [.041;.054]** | *.042* [.036;.048] |
| | PT:SM | .245 [.232;.259] | **.048 [.042;.055]** | .062 [.055;.070] | **.051 [.044;.058]** | **.045 [.039;.052]** |
| As:Am:Aps | no PT:SM | .220 [.208;.233] | *.042* [.036;.049] | **.054 [.047;.061]** | **.048 [.042;.055]** | *.041* [.036;.048] |
| | PT:SM | .232 [.219;.245] | **.048 [.041;.055]** | .061 [.054;.069] | **.048 [.042;.055]** | **.048 [.041;.055]** |
| Ap:As:Am:Aps | no PT:SM | .133 [.123;.144] | **.051 [.045;.059]** | **.054 [.047;.061]** | *.043* [.037;.050] | **.049 [.043;.056]** |
| | PT:SM | .124 [.114;.134] | **.046 [.039;.052]** | **.045 [.039;.052]** | *.040* [.034;.046] | *.043* [.037;.050] |

Table S21: Type I error rate of the model M4 (see Table 2): The data are simulated using correlated random effects, 18 participants, and 18 stimuli. Represented are the models that do not include random effects associated to the interaction participants:stimuli.

| | | RI | RI-L | ZCP-sum | ZCP-poly | gANOVA |
|---|---|---|---|---|---|---|
| Ap | no PT:SM | .077 [.069;.086] | **.044 [.039;.051]** | **.047 [.040;.054]** | **.047 [.041;.054]** | **.047 [.041;.054]** |
| | PT:SM | .080 [.072;.089] | **.050 [.044;.058]** | **.051 [.044;.058]** | **.053 [.047;.061]** | **.052 [.046;.060]** |
| As | no PT:SM | .102 [.094;.112] | **.051 [.045;.059]** | **.053 [.046;.060]** | **.053 [.047;.061]** | **.054 [.048;.062]** |
| | PT:SM | .096 [.088;.106] | **.050 [.044;.058]** | **.048 [.042;.056]** | **.055 [.048;.063]** | **.052 [.046;.060]** |
| Am | no PT:SM | .504 [.489;.520] | **.050 [.044;.058]** | .062 [.055;.070] | .058 [.051;.066] | **.050 [.043;.057]** |
| | PT:SM | .532 [.517;.548] | .057 [.050;.065] | .070 [.062;.078] | .062 [.055;.070] | .057 [.050;.065] |
| Aps | no PT:SM | .410 [.395;.426] | **.045 [.039;.052]** | **.046 [.040;.053]** | **.044 [.038;.051]** | **.044 [.038;.051]** |
| | PT:SM | .420 [.405;.435] | *.042* [.036;.049] | **.044 [.039;.051]** | *.042* [.037;.049] | *.041* [.035;.048] |
| Ap:As | no PT:SM | .796 [.783;.808] | **.046 [.040;.054]** | **.049 [.042;.056]** | **.050 [.043;.057]** | **.045 [.039;.052]** |
| | PT:SM | .816 [.804;.828] | **.051 [.045;.059]** | **.045 [.039;.052]** | **.053 [.046;.060]** | **.050 [.043;.057]** |
| Ap:Am | no PT:SM | .536 [.521;.552] | .056 [.050;.064] | .075 [.068;.084] | .064 [.056;.072] | .056 [.050;.064] |
| | PT:SM | .602 [.587;.617] | **.048 [.042;.055]** | .072 [.064;.080] | .058 [.051;.066] | **.048 [.042;.055]** |
| Ap:Aps | no PT:SM | .479 [.464;.494] | *.043* [.037;.050] | **.044 [.038;.051]** | *.041* [.035;.048] | *.040* [.034;.046] |
| | PT:SM | .508 [.493;.524] | **.050 [.044;.057]** | **.048 [.041;.055]** | **.052 [.045;.059]** | **.050 [.044;.057]** |
| As:Am | no PT:SM | .473 [.458;.489] | .065 [.058;.073] | .086 [.078;.095] | .070 [.062;.078] | .063 [.056;.071] |
| | PT:SM | .550 [.535;.565] | .056 [.050;.064] | .082 [.074;.091] | .066 [.058;.074] | **.056 [.049;.063]** |
| As:Aps | no PT:SM | .459 [.444;.475] | **.048 [.042;.055]** | **.044 [.038;.051]** | **.046 [.040;.053]** | **.046 [.040;.053]** |
| | PT:SM | .472 [.457;.488] | **.055 [.048;.063]** | **.056 [.049;.063]** | **.055 [.048;.063]** | **.056 [.049;.063]** |
| Am:Aps | no PT:SM | .146 [.135;.157] | .058 [.052;.066] | .075 [.068;.084] | .064 [.057;.072] | .059 [.052;.067] |
| | PT:SM | .188 [.177;.201] | **.049 [.043;.056]** | .068 [.060;.076] | .057 [.050;.065] | **.050 [.043;.057]** |
| Ap:As:Am | no PT:SM | .200 [.187;.212] | .067 [.060;.075] | .123 [.113;.133] | .086 [.078;.096] | .069 [.062;.077] |
| | PT:SM | .265 [.252;.279] | **.055 [.048;.063]** | .106 [.097;.116] | .074 [.066;.083] | **.056 [.049;.063]** |
| Ap:As:Aps | no PT:SM | .384 [.370;.400] | *.031* [.026;.037] | *.040* [.034;.047] | *.040* [.034;.046] | *.030* [.025;.035] |
| | PT:SM | .362 [.347;.377] | *.038* [.033;.044] | **.054 [.048;.062]** | **.048 [.042;.055]** | *.038* [.033;.044] |
| Ap:Am:Aps | no PT:SM | .114 [.104;.124] | **.052 [.045;.059]** | .073 [.065;.081] | **.054 [.048;.062]** | **.052 [.046;.060]** |
| | PT:SM | .147 [.137;.159] | **.046 [.040;.054]** | .070 [.062;.078] | **.051 [.045;.058]** | **.047 [.041;.054]** |
| As:Am:Aps | no PT:SM | .104 [.094;.113] | .059 [.052;.067] | .073 [.065;.082] | **.056 [.049;.064]** | .059 [.052;.067] |
| | PT:SM | .150 [.140;.162] | .057 [.050;.065] | .079 [.071;.088] | .060 [.053;.068] | .057 [.050;.065] |
| Ap:As:Am:Aps | no PT:SM | *.036* [.031;.043] | .069 [.061;.077] | .066 [.058;.074] | **.048 [.042;.055]** | .066 [.059;.075] |
| | PT:SM | .067 [.059;.075] | **.052 [.046;.060]** | .078 [.070;.087] | *.043* [.037;.050] | **.050 [.044;.058]** |

Table S22: Type I error rate of the model M4 (see Table 2): The data are simulated using correlated random effects, 18 participants, and 18 stimuli. Represented are the models that include random effects associated to the interaction participants:stimuli.

| | | RI+ | RI-L+ | ZCP-sum+ | ZCP-poly+ | gANOVA+ |
|---|---|---|---|---|---|---|
| Ap | no PT:SM | .077 [.069;.085] | **.046 [.039;.052]** | **.047 [.041;.054]** | **.050 [.043;.057]** | **.050 [.044;.058]** |
| | PT:SM | .080 [.072;.089] | **.051 [.045;.058]** | **.051 [.045;.058]** | **.054 [.047;.061]** | **.052 [.046;.060]** |
| As | no PT:SM | .102 [.093;.112] | **.054 [.047;.061]** | .057 [.050;.065] | .059 [.052;.067] | .057 [.050;.065] |
| | PT:SM | .097 [.088;.107] | **.051 [.044;.058]** | **.049 [.043;.056]** | **.055 [.049;.063]** | **.053 [.047;.061]** |
| Am | no PT:SM | .595 [.580;.611] | **.048 [.042;.055]** | .058 [.051;.066] | **.054 [.047;.061]** | **.046 [.040;.053]** |
| | PT:SM | .593 [.578;.608] | .057 [.050;.064] | .070 [.062;.078] | .062 [.055;.070] | .057 [.050;.064] |
| Aps | no PT:SM | .305 [.291;.319] | **.049 [.043;.056]** | **.050 [.044;.057]** | **.048 [.042;.055]** | **.048 [.042;.055]** |
| | PT:SM | .346 [.331;.361] | *.042* [.037;.049] | **.045 [.039;.052]** | *.043* [.037;.050] | *.041* [.036;.048] |
| Ap:As | no PT:SM | .623 [.608;.638] | **.051 [.044;.058]** | **.055 [.049;.063]** | .058 [.051;.066] | **.050 [.043;.057]** |
| | PT:SM | .698 [.684;.713] | **.052 [.046;.059]** | **.045 [.039;.052]** | **.053 [.047;.061]** | **.050 [.044;.057]** |
| Ap:Am | no PT:SM | .670 [.656;.685] | **.052 [.046;.059]** | .072 [.064;.080] | .060 [.053;.068] | **.052 [.045;.059]** |
| | PT:SM | .686 [.671;.700] | **.048 [.042;.055]** | .072 [.064;.080] | .058 [.051;.065] | **.047 [.041;.054]** |
| Ap:Aps | no PT:SM | .318 [.304;.333] | **.048 [.042;.055]** | **.046 [.040;.053]** | **.046 [.039;.052]** | **.044 [.038;.051]** |
| | PT:SM | .390 [.375;.405] | **.050 [.044;.058]** | **.048 [.042;.055]** | **.052 [.046;.060]** | **.051 [.044;.058]** |
| As:Am | no PT:SM | .626 [.611;.641] | .056 [.050;.064] | .081 [.073;.090] | .064 [.057;.072] | .056 [.050;.064] |
| | PT:SM | .636 [.622;.652] | **.055 [.048;.063]** | .081 [.073;.090] | .065 [.058;.073] | **.054 [.048;.062]** |
| As:Aps | no PT:SM | .303 [.289;.318] | **.056 [.049;.063]** | .056 [.050;.064] | **.054 [.048;.062]** | **.055 [.048;.062]** |
| | PT:SM | .361 [.346;.376] | **.056 [.049;.063]** | .057 [.050;.065] | **.056 [.049;.063]** | **.056 [.049;.064]** |
| Am:Aps | no PT:SM | .238 [.225;.252] | **.052 [.045;.059]** | .072 [.064;.080] | **.055 [.048;.062]** | **.052 [.046;.059]** |
| | PT:SM | .260 [.247;.274] | **.049 [.043;.056]** | .066 [.059;.074] | .056 [.050;.064] | **.050 [.043;.057]** |
| Ap:As:Am | no PT:SM | .396 [.381;.411] | **.056 [.049;.063]** | .114 [.104;.124] | .074 [.066;.082] | .056 [.050;.064] |
| | PT:SM | .409 [.394;.424] | **.054 [.047;.061]** | .105 [.096;.115] | .074 [.066;.082] | **.054 [.047;.061]** |
| Ap:As:Aps | no PT:SM | .181 [.169;.193] | **.046 [.040;.054]** | **.053 [.046;.060]** | .059 [.052;.067] | **.049 [.043;.056]** |
| | PT:SM | .200 [.188;.213] | *.039* [.034;.046] | **.055 [.048;.063]** | **.050 [.043;.057]** | *.040* [.035;.047] |
| Ap:Am:Aps | no PT:SM | .238 [.225;.252] | **.044 [.038;.051]** | .072 [.064;.080] | **.049 [.043;.056]** | **.044 [.039;.051]** |
| | PT:SM | .236 [.224;.250] | **.046 [.040;.053]** | .068 [.061;.077] | **.051 [.044;.058]** | **.046 [.040;.054]** |
| As:Am:Aps | no PT:SM | .219 [.207;.232] | **.050 [.043;.057]** | .071 [.063;.079] | **.054 [.047;.061]** | **.050 [.043;.057]** |
| | PT:SM | .232 [.220;.246] | **.056 [.049;.064]** | .079 [.071;.088] | .059 [.052;.067] | **.055 [.048;.062]** |
| Ap:As:Am:Aps | no PT:SM | .134 [.124;.145] | **.056 [.049;.063]** | .077 [.069;.085] | **.045 [.039;.052]** | **.052 [.046;.059]** |
| | PT:SM | .152 [.142;.164] | **.052 [.045;.059]** | .078 [.071;.087] | *.042* [.036;.048] | **.049 [.043;.056]** |

# 2 Results of simulation: power analysis

Table S23: Power analysis of model M2 (see Table 2): The data are simulated using spherical random effects, without the interaction participants:stimuli. The estimated models do not include the random effects associated to the interaction participants:stimuli.

| variable | model | H0 | 0.2 | 0.4 | 0.6 | 0.8 | 1.0 |
|---|---|---|---|---|---|---|---|
| Ap | RI | .074 [.067;.083] | .146 [.136;.158] | .383 [.368;.399] | .713 [.699;.727] | .922 [.913;.930] | .989 [.986;.992] |
| | RI-L | .052 [.046;.059] | .112 [.103;.122] | .318 [.304;.333] | .658 [.643;.672] | .897 [.888;.906] | .984 [.980;.987] |
| | ZCP-sum | .052 [.045;.059] | .099 [.090;.109] | .280 [.266;.294] | .607 [.592;.622] | .872 [.862;.883] | .977 [.973;.982] |
| | ZCP-poly | .054 [.047;.061] | .112 [.103;.122] | .318 [.303;.332] | .659 [.644;.674] | .897 [.888;.907] | .983 [.980;.987] |
| | gANOVA | .052 [.046;.060] | .112 [.102;.122] | .318 [.304;.333] | .658 [.643;.672] | .897 [.888;.906] | .984 [.980;.987] |
| As | RI | .086 [.078;.096] | .183 [.172;.196] | .468 [.453;.484] | .784 [.771;.797] | .951 [.945;.958] | .996 [.994;.998] |
| | RI-L | .051 [.045;.059] | .122 [.113;.133] | .377 [.363;.393] | .712 [.699;.727] | .928 [.920;.936] | .992 [.990;.995] |
| | ZCP-sum | .047 [.041;.054] | .104 [.095;.114] | .324 [.310;.339] | .655 [.640;.670] | .903 [.894;.912] | .988 [.984;.991] |
| | ZCP-poly | .052 [.045;.059] | .124 [.114;.135] | .377 [.362;.392] | .710 [.696;.724] | .928 [.920;.936] | .992 [.990;.995] |
| | gANOVA | .051 [.045;.059] | .122 [.113;.133] | .377 [.363;.393] | .712 [.698;.726] | .928 [.920;.936] | .992 [.990;.995] |
| Am | RI | .463 [.448;.479] | .632 [.617;.647] | .891 [.881;.901] | .986 [.983;.990] | 1 [.999;1] | 1 [1;1] |
| | RI-L | .051 [.045;.059] | .146 [.135;.157] | .451 [.436;.467] | .812 [.800;.824] | .971 [.966;.976] | .998 [.997;1] |
| | ZCP-sum | .075 [.067;.083] | .130 [.119;.140] | .328 [.313;.342] | .651 [.636;.666] | .903 [.894;.912] | .984 [.980;.987] |
| | ZCP-poly | .056 [.049;.063] | .154 [.143;.166] | .459 [.443;.474] | .809 [.797;.821] | .966 [.961;.972] | .998 [.996;.999] |
| | gANOVA | .051 [.045;.059] | .146 [.135;.157] | .450 [.435;.466] | .812 [.799;.824] | .971 [.966;.976] | .998 [.997;1] |
| Ap:As | RI | .814 [.803;.827] | .863 [.852;.874] | .942 [.935;.949] | .984 [.980;.988] | .998 [.997;.999] | 1 [.999;1] |
| | RI-L | .042 [.036;.048] | .073 [.065;.081] | .194 [.182;.207] | .428 [.413;.444] | .704 [.690;.718] | .908 [.899;.917] |
| | ZCP-sum | .046 [.040;.053] | .056 [.049;.063] | .101 [.092;.111] | .212 [.200;.225] | .413 [.398;.428] | .658 [.643;.672] |
| | ZCP-poly | .046 [.040;.053] | .080 [.072;.088] | .197 [.185;.209] | .433 [.418;.448] | .701 [.687;.715] | .898 [.889;.908] |
| | gANOVA | .042 [.036;.048] | .073 [.065;.081] | .194 [.182;.207] | .427 [.412;.443] | .702 [.688;.716] | .906 [.898;.916] |
| Ap:Am | RI | .467 [.452;.482] | .582 [.566;.597] | .788 [.775;.800] | .936 [.929;.944] | .994 [.991;.996] | 1 [1;1] |
| | RI-L | .056 [.049;.063] | .100 [.091;.110] | .266 [.252;.280] | .545 [.530;.560] | .814 [.802;.826] | .954 [.947;.960] |
| | ZCP-sum | .076 [.068;.084] | .095 [.087;.105] | .186 [.174;.198] | .367 [.352;.382] | .612 [.597;.627] | .820 [.808;.832] |
| | ZCP-poly | .066 [.058;.074] | .104 [.095;.114] | .269 [.255;.283] | .537 [.522;.553] | .804 [.792;.816] | .948 [.942;.955] |
| | gANOVA | .056 [.049;.063] | .100 [.091;.110] | .265 [.251;.279] | .544 [.529;.560] | .814 [.802;.826] | .954 [.947;.960] |
| As:Am | RI | .408 [.394;.424] | .572 [.557;.588] | .862 [.852;.873] | .984 [.980;.988] | .999 [.998;1] | 1 [1;1] |
| | RI-L | .062 [.055;.070] | .126 [.116;.136] | .408 [.393;.424] | .785 [.772;.798] | .963 [.957;.969] | .998 [.997;1] |
| | ZCP-sum | .078 [.071;.087] | .120 [.111;.131] | .283 [.270;.298] | .575 [.560;.591] | .864 [.854;.875] | .975 [.970;.980] |
| | ZCP-poly | .068 [.061;.076] | .134 [.123;.145] | .414 [.399;.430] | .774 [.761;.787] | .958 [.952;.965] | .999 [.998;1] |
| | gANOVA | .062 [.054;.069] | .126 [.116;.136] | .407 [.392;.422] | .784 [.772;.797] | .963 [.957;.969] | .998 [.997;1] |
| Ap:As:Am | RI | .109 [.100;.119] | .150 [.139;.161] | .257 [.244;.271] | .465 [.450;.480] | .705 [.691;.719] | .890 [.881;.900] |
| | RI-L | .080 [.072;.088] | .100 [.091;.110] | .185 [.173;.197] | .350 [.336;.366] | .581 [.566;.596] | .804 [.792;.816] |
| | ZCP-sum | .072 [.064;.080] | .083 [.075;.092] | .131 [.121;.142] | .241 [.228;.254] | .407 [.392;.422] | .610 [.595;.625] |
| | ZCP-poly | .070 [.063;.079] | .091 [.083;.100] | .165 [.154;.177] | .322 [.307;.336] | .556 [.541;.572] | .777 [.764;.790] |
| | gANOVA | .080 [.072;.088] | .100 [.092;.110] | .185 [.173;.197] | .350 [.336;.366] | .581 [.566;.596] | .804 [.792;.816] |

Table S24: Power analysis of model M2 (see Table 2): The data are simulated using spherical random effects, without the interaction participants:stimuli. The estimated models do not include the random effects associated to the interaction participants:stimuli.

| variable | model | H0 | 0.2 | 0.4 | 0.6 | 0.8 | 1.0 |
|---|---|---|---|---|---|---|---|
| Ap | RI | .074 [.067;.083] | .146 [.136;.158] | .383 [.368;.399] | .713 [.699;.727] | .922 [.913;.930] | .989 [.986;.992] |
| | RI-L | .054 [.047;.061] | .116 [.106;.126] | .325 [.311;.340] | .662 [.648;.677] | .900 [.890;.909] | .985 [.981;.989] |
| | ZCP-sum | .056 [.049;.063] | .105 [.096;.115] | .296 [.282;.310] | .621 [.606;.636] | .881 [.871;.891] | .980 [.975;.984] |
| | ZCP-poly | .055 [.048;.063] | .114 [.105;.125] | .324 [.310;.339] | .662 [.648;.677] | .900 [.891;.910] | .985 [.981;.989] |
| | gANOVA | .054 [.048;.062] | .115 [.106;.126] | .324 [.310;.339] | .662 [.648;.677] | .900 [.890;.909] | .985 [.981;.989] |
| As | RI | .086 [.078;.096] | .183 [.172;.196] | .468 [.453;.484] | .784 [.771;.797] | .951 [.945;.958] | .996 [.994;.998] |
| | RI-L | .052 [.046;.060] | .126 [.116;.136] | .385 [.370;.400] | .718 [.704;.732] | .930 [.922;.938] | .993 [.990;.996] |
| | ZCP-sum | .052 [.045;.059] | .112 [.102;.122] | .339 [.325;.354] | .669 [.654;.683] | .908 [.899;.917] | .989 [.985;.992] |
| | ZCP-poly | .055 [.048;.063] | .128 [.118;.139] | .384 [.370;.400] | .716 [.703;.731] | .930 [.922;.937] | .993 [.990;.995] |
| | gANOVA | .052 [.046;.060] | .125 [.115;.136] | .385 [.370;.400] | .718 [.704;.732] | .930 [.922;.938] | .993 [.990;.996] |
| Am | RI | .550 [.535;.566] | .702 [.688;.717] | .920 [.912;.929] | .991 [.988;.994] | 1 [.999;1] | 1 [1;1] |
| | RI-L | .047 [.041;.054] | .136 [.126;.147] | .437 [.422;.452] | .803 [.791;.816] | .968 [.963;.974] | .998 [.996;.999] |
| | ZCP-sum | .071 [.063;.079] | .117 [.107;.127] | .297 [.283;.311] | .612 [.597;.627] | .885 [.875;.895] | .980 [.975;.984] |
| | ZCP-poly | .051 [.045;.059] | .147 [.136;.158] | .447 [.432;.463] | .799 [.787;.812] | .965 [.959;.971] | .998 [.996;.999] |
| | gANOVA | .047 [.041;.054] | .136 [.126;.147] | .436 [.421;.452] | .802 [.790;.815] | .968 [.963;.974] | .998 [.996;.999] |
| Ap:As | RI | .673 [.658;.687] | .732 [.719;.746] | .871 [.860;.881] | .962 [.956;.968] | .993 [.991;.996] | 1 [.999;1] |
| | RI-L | .048 [.042;.055] | .084 [.076;.093] | .212 [.200;.225] | .450 [.435;.466] | .723 [.710;.737] | .915 [.907;.924] |
| | ZCP-sum | .055 [.048;.063] | .069 [.062;.077] | .124 [.115;.135] | .261 [.247;.275] | .476 [.461;.492] | .715 [.701;.729] |
| | ZCP-poly | .054 [.047;.061] | .090 [.081;.099] | .218 [.205;.231] | .455 [.440;.470] | .723 [.709;.737] | .905 [.896;.914] |
| | gANOVA | .048 [.042;.055] | .084 [.075;.093] | .212 [.199;.225] | .448 [.433;.464] | .721 [.707;.735] | .915 [.906;.924] |
| Ap:Am | RI | .608 [.593;.623] | .696 [.682;.710] | .857 [.846;.868] | .965 [.960;.971] | .998 [.997;.999] | 1 [1;1] |
| | RI-L | .048 [.042;.056] | .091 [.083;.101] | .243 [.230;.257] | .518 [.503;.534] | .798 [.785;.810] | .946 [.939;.953] |
| | ZCP-sum | .072 [.064;.080] | .087 [.078;.096] | .165 [.154;.177] | .328 [.314;.343] | .569 [.554;.585] | .793 [.781;.806] |
| | ZCP-poly | .058 [.051;.066] | .093 [.085;.103] | .252 [.239;.266] | .521 [.506;.537] | .792 [.779;.804] | .944 [.937;.952] |
| | gANOVA | .048 [.042;.055] | .091 [.083;.101] | .242 [.229;.256] | .518 [.503;.534] | .797 [.785;.810] | .946 [.939;.953] |
| As:Am | RI | .543 [.528;.559] | .697 [.683;.711] | .914 [.906;.923] | .991 [.988;.994] | 1 [1;1] | 1 [1;1] |
| | RI-L | .054 [.047;.061] | .110 [.100;.120] | .378 [.363;.393] | .760 [.747;.774] | .959 [.953;.965] | .998 [.997;.999] |
| | ZCP-sum | .072 [.064;.080] | .106 [.097;.116] | .245 [.232;.259] | .522 [.507;.538] | .830 [.818;.841] | .965 [.959;.970] |
| | ZCP-poly | .061 [.054;.069] | .122 [.112;.132] | .391 [.376;.406] | .754 [.741;.768] | .956 [.949;.962] | .998 [.996;.999] |
| | gANOVA | .054 [.047;.061] | .110 [.100;.120] | .378 [.363;.393] | .759 [.746;.773] | .959 [.953;.965] | .998 [.997;.999] |
| Ap:As:Am | RI | .261 [.247;.275] | .310 [.296;.325] | .460 [.445;.476] | .666 [.652;.681] | .858 [.848;.869] | .954 [.948;.961] |
| | RI-L | .052 [.046;.060] | .069 [.062;.077] | .136 [.126;.147] | .283 [.270;.298] | .507 [.492;.523] | .741 [.728;.755] |
| | ZCP-sum | .071 [.063;.079] | .079 [.071;.088] | .115 [.106;.125] | .195 [.183;.207] | .329 [.314;.343] | .510 [.495;.526] |
| | ZCP-poly | .060 [.053;.068] | .078 [.070;.087] | .143 [.132;.154] | .292 [.278;.306] | .509 [.494;.525] | .739 [.726;.753] |
| | gANOVA | .052 [.046;.060] | .069 [.062;.077] | .136 [.126;.148] | .284 [.270;.298] | .507 [.492;.523] | .741 [.728;.755] |

Table S25: Power analysis of model M2 (see Table 2): The data are simulated using spherical random effects, with the interaction participants:stimuli. The estimated models do not include the random effects associated to the interaction participants:stimuli.

| variable | model | H0 | 0.2 | 0.4 | 0.6 | 0.8 | 1.0 |
|---|---|---|---|---|---|---|---|
| Ap | RI | .075 [.067;.084] | .152 [.141;.164] | .410 [.395;.425] | .738 [.724;.751] | .935 [.928;.943] | .991 [.988;.994] |
| | RI-L | .056 [.049;.063] | .117 [.107;.127] | .350 [.335;.365] | .686 [.672;.701] | .918 [.910;.927] | .986 [.983;.990] |
| | ZCP-sum | .054 [.047;.061] | .109 [.100;.119] | .312 [.298;.327] | .642 [.627;.657] | .892 [.882;.901] | .984 [.980;.987] |
| | ZCP-poly | .055 [.048;.063] | .120 [.110;.130] | .350 [.335;.365] | .686 [.672;.701] | .918 [.910;.927] | .986 [.983;.990] |
| | gANOVA | .056 [.049;.064] | .117 [.107;.127] | .350 [.335;.365] | .686 [.672;.701] | .918 [.910;.927] | .986 [.983;.990] |
| As | RI | .088 [.079;.097] | .190 [.179;.203] | .478 [.463;.494] | .798 [.786;.811] | .962 [.956;.968] | .996 [.994;.998] |
| | RI-L | .053 [.046;.060] | .128 [.118;.139] | .394 [.379;.409] | .738 [.725;.752] | .943 [.936;.950] | .994 [.992;.996] |
| | ZCP-sum | .050 [.043;.057] | .111 [.102;.121] | .339 [.325;.354] | .675 [.661;.690] | .922 [.913;.930] | .990 [.987;.993] |
| | ZCP-poly | .052 [.046;.060] | .128 [.118;.139] | .394 [.379;.409] | .736 [.723;.750] | .942 [.935;.949] | .994 [.992;.996] |
| | gANOVA | .053 [.046;.060] | .128 [.118;.139] | .394 [.379;.409] | .738 [.725;.752] | .943 [.936;.950] | .994 [.992;.996] |
| Am | RI | .515 [.500;.531] | .680 [.665;.694] | .909 [.900;.918] | .991 [.988;.994] | 1 [.999;1] | 1 [1;1] |
| | RI-L | .046 [.040;.054] | .141 [.131;.152] | .440 [.425;.456] | .803 [.791;.815] | .970 [.965;.976] | .999 [.998;1] |
| | ZCP-sum | .070 [.062;.078] | .108 [.099;.118] | .282 [.269;.297] | .607 [.592;.623] | .888 [.878;.898] | .983 [.979;.987] |
| | ZCP-poly | .053 [.046;.060] | .145 [.134;.156] | .441 [.426;.457] | .795 [.783;.808] | .970 [.964;.975] | .999 [.998;1] |
| | gANOVA | .046 [.040;.054] | .141 [.131;.152] | .440 [.425;.456] | .803 [.791;.815] | .970 [.965;.976] | .999 [.998;1] |
| Ap:As | RI | .843 [.832;.854] | .884 [.874;.894] | .948 [.941;.955] | .987 [.983;.990] | 1 [.999;1] | 1 [1;1] |
| | RI-L | .049 [.043;.056] | .087 [.079;.096] | .230 [.217;.243] | .484 [.469;.500] | .763 [.750;.776] | .929 [.921;.937] |
| | ZCP-sum | .047 [.041;.054] | .062 [.055;.070] | .111 [.102;.121] | .254 [.241;.268] | .467 [.452;.483] | .720 [.706;.734] |
| | ZCP-poly | .058 [.051;.065] | .094 [.086;.104] | .234 [.221;.248] | .494 [.479;.510] | .761 [.748;.774] | .928 [.919;.936] |
| | gANOVA | .048 [.042;.055] | .087 [.078;.096] | .229 [.217;.243] | .483 [.468;.498] | .762 [.749;.776] | .929 [.921;.937] |
| Ap:Am | RI | .558 [.542;.573] | .662 [.648;.677] | .840 [.828;.851] | .958 [.951;.964] | .994 [.991;.996] | 1 [.999;1] |
| | RI-L | .049 [.043;.056] | .095 [.087;.105] | .247 [.234;.260] | .522 [.507;.538] | .800 [.788;.813] | .949 [.942;.956] |
| | ZCP-sum | .064 [.056;.072] | .088 [.080;.098] | .162 [.151;.174] | .327 [.313;.342] | .572 [.557;.587] | .791 [.778;.803] |
| | ZCP-poly | .059 [.052;.067] | .099 [.090;.109] | .257 [.244;.271] | .532 [.517;.548] | .791 [.779;.804] | .944 [.937;.951] |
| | gANOVA | .049 [.043;.056] | .095 [.086;.105] | .246 [.234;.260] | .522 [.506;.537] | .800 [.787;.812] | .949 [.942;.956] |
| As:Am | RI | .496 [.480;.511] | .646 [.632;.661] | .893 [.884;.903] | .989 [.985;.992] | 1 [1;1] | 1 [1;1] |
| | RI-L | .053 [.046;.060] | .121 [.111;.132] | .380 [.365;.395] | .757 [.744;.770] | .953 [.946;.959] | .997 [.995;.999] |
| | ZCP-sum | .067 [.060;.075] | .102 [.093;.112] | .244 [.231;.258] | .521 [.505;.536] | .813 [.801;.825] | .960 [.954;.966] |
| | ZCP-poly | .054 [.048;.062] | .132 [.122;.143] | .388 [.374;.404] | .756 [.743;.770] | .948 [.942;.955] | .998 [.996;.999] |
| | gANOVA | .053 [.046;.060] | .121 [.111;.131] | .380 [.365;.395] | .756 [.743;.769] | .952 [.946;.959] | .997 [.995;.999] |
| Ap:As:Am | RI | .190 [.178;.203] | .235 [.222;.249] | .380 [.366;.396] | .596 [.580;.611] | .808 [.796;.821] | .941 [.934;.948] |
| | RI-L | .050 [.044;.057] | .071 [.063;.079] | .140 [.130;.151] | .292 [.279;.307] | .516 [.500;.531] | .754 [.741;.768] |
| | ZCP-sum | .072 [.064;.080] | .086 [.078;.095] | .122 [.112;.132] | .199 [.187;.212] | .334 [.320;.349] | .512 [.497;.528] |
| | ZCP-poly | .064 [.057;.072] | .084 [.075;.093] | .159 [.148;.171] | .308 [.294;.322] | .527 [.512;.543] | .754 [.741;.768] |
| | gANOVA | .050 [.044;.057] | .071 [.063;.079] | .140 [.130;.151] | .292 [.278;.307] | .516 [.501;.532] | .754 [.741;.767] |

Table S26: Power analysis of model M2 (see Table 2): The data are simulated using spherical random effects, with the interaction participants:stimuli. The estimated models include the random effects associated to the interaction participants:stimuli.

| variable | model | H0 | 0.2 | 0.4 | 0.6 | 0.8 | 1.0 |
|---|---|---|---|---|---|---|---|
| Ap | RI | .075 [.067;.084] | .152 [.141;.164] | .410 [.395;.425] | .738 [.724;.751] | .935 [.928;.943] | .991 [.988;.994] |
| | RI-L | .056 [.049;.063] | .117 [.108;.127] | .350 [.336;.365] | .686 [.672;.701] | .918 [.910;.927] | .986 [.983;.990] |
| | ZCP-sum | .054 [.047;.061] | .109 [.100;.119] | .312 [.298;.327] | .644 [.629;.659] | .892 [.883;.902] | .984 [.980;.988] |
| | ZCP-poly | .056 [.049;.063] | .120 [.110;.130] | .351 [.336;.366] | .686 [.672;.701] | .918 [.910;.927] | .987 [.983;.990] |
| | gANOVA | .056 [.049;.064] | .117 [.107;.127] | .350 [.335;.365] | .686 [.672;.701] | .918 [.910;.927] | .986 [.983;.990] |
| As | RI | .088 [.079;.097] | .190 [.179;.203] | .478 [.463;.494] | .798 [.786;.811] | .962 [.956;.968] | .996 [.994;.998] |
| | RI-L | .053 [.047;.060] | .129 [.119;.140] | .395 [.380;.410] | .739 [.725;.753] | .943 [.936;.950] | .994 [.992;.996] |
| | ZCP-sum | .051 [.045;.058] | .112 [.102;.122] | .341 [.327;.356] | .676 [.662;.691] | .922 [.914;.931] | .990 [.987;.993] |
| | ZCP-poly | .053 [.046;.060] | .128 [.118;.139] | .394 [.379;.409] | .737 [.723;.751] | .942 [.935;.950] | .994 [.992;.996] |
| | gANOVA | .053 [.046;.060] | .129 [.119;.140] | .395 [.380;.410] | .739 [.725;.752] | .943 [.936;.950] | .994 [.992;.996] |
| Am | RI | .560 [.545;.576] | .709 [.695;.723] | .924 [.916;.932] | .992 [.989;.995] | 1 [.999;1] | 1 [1;1] |
| | RI-L | .046 [.040;.053] | .140 [.130;.152] | .439 [.424;.455] | .801 [.789;.814] | .970 [.965;.975] | .999 [.998;1] |
| | ZCP-sum | .069 [.062;.078] | .108 [.098;.118] | .282 [.268;.296] | .606 [.591;.621] | .887 [.877;.897] | .983 [.979;.987] |
| | ZCP-poly | .052 [.046;.059] | .144 [.134;.156] | .441 [.426;.457] | .795 [.783;.808] | .970 [.964;.975] | .999 [.998;1] |
| | gANOVA | .046 [.040;.053] | .140 [.130;.151] | .439 [.424;.455] | .802 [.789;.814] | .970 [.965;.976] | .999 [.998;1] |
| Ap:As | RI | .777 [.764;.790] | .831 [.819;.843] | .926 [.918;.934] | .978 [.973;.982] | .997 [.996;.999] | 1 [1;1] |
| | RI-L | .049 [.043;.056] | .088 [.079;.097] | .231 [.218;.244] | .485 [.470;.501] | .764 [.751;.777] | .930 [.922;.938] |
| | ZCP-sum | .047 [.041;.054] | .062 [.055;.070] | .113 [.104;.124] | .257 [.244;.271] | .472 [.457;.488] | .724 [.710;.738] |
| | ZCP-poly | .058 [.051;.066] | .095 [.087;.105] | .236 [.223;.250] | .496 [.480;.511] | .763 [.750;.776] | .928 [.920;.936] |
| | gANOVA | .048 [.042;.056] | .087 [.079;.096] | .230 [.217;.243] | .484 [.469;.499] | .763 [.750;.776] | .930 [.922;.938] |
| Ap:Am | RI | .623 [.608;.638] | .714 [.700;.728] | .871 [.861;.882] | .967 [.962;.973] | .996 [.994;.998] | 1 [.999;1] |
| | RI-L | .048 [.041;.055] | .095 [.086;.104] | .245 [.232;.259] | .521 [.506;.537] | .800 [.787;.812] | .949 [.942;.956] |
| | ZCP-sum | .063 [.056;.071] | .088 [.080;.098] | .162 [.150;.173] | .327 [.312;.341] | .570 [.555;.585] | .789 [.776;.802] |
| | ZCP-poly | .058 [.051;.065] | .099 [.090;.109] | .255 [.242;.269] | .530 [.515;.546] | .790 [.777;.803] | .944 [.937;.951] |
| | gANOVA | .048 [.041;.055] | .094 [.086;.104] | .245 [.232;.259] | .521 [.505;.536] | .799 [.787;.812] | .948 [.942;.955] |
| As:Am | RI | .560 [.544;.575] | .702 [.688;.717] | .916 [.907;.924] | .993 [.990;.996] | 1 [1;1] | 1 [1;1] |
| | RI-L | .052 [.046;.060] | .120 [.111;.131] | .378 [.364;.394] | .755 [.742;.769] | .952 [.946;.959] | .997 [.995;.999] |
| | ZCP-sum | .067 [.060;.075] | .102 [.093;.112] | .241 [.228;.254] | .518 [.502;.533] | .811 [.799;.823] | .959 [.953;.965] |
| | ZCP-poly | .054 [.048;.062] | .131 [.121;.142] | .388 [.373;.404] | .755 [.742;.768] | .948 [.941;.955] | .998 [.996;.999] |
| | gANOVA | .052 [.046;.060] | .120 [.110;.130] | .378 [.364;.394] | .754 [.741;.768] | .952 [.945;.959] | .997 [.995;.999] |
| Ap:As:Am | RI | .271 [.257;.285] | .327 [.313;.342] | .477 [.462;.493] | .690 [.676;.705] | .867 [.856;.877] | .964 [.958;.970] |
| | RI-L | .048 [.042;.055] | .069 [.061;.077] | .136 [.126;.147] | .288 [.274;.302] | .512 [.496;.527] | .748 [.735;.762] |
| | ZCP-sum | .071 [.063;.079] | .086 [.078;.095] | .120 [.111;.131] | .197 [.185;.210] | .329 [.315;.344] | .506 [.490;.521] |
| | ZCP-poly | .063 [.056;.071] | .084 [.075;.093] | .157 [.146;.169] | .304 [.290;.319] | .524 [.509;.540] | .751 [.737;.764] |
| | gANOVA | .048 [.042;.055] | .068 [.061;.077] | .136 [.126;.147] | .288 [.274;.302] | .511 [.496;.527] | .748 [.735;.762] |

Table S27: Power analysis of model M2 (see Table 2): The data are simulated using correlated random effects, without the interaction participants:stimuli. The estimated models do not include the random effects associated to the interaction participants:stimuli.

| variable | model | H0 | 0.2 | 0.4 | 0.6 | 0.8 | 1.0 |
|---|---|---|---|---|---|---|---|
| Ap | RI | .076 [.069;.085] | .169 [.158;.181] | .390 [.375;.405] | .706 [.692;.720] | .910 [.901;.919] | .990 [.987;.993] |
| | RI-L | .051 [.045;.059] | .131 [.121;.142] | .340 [.325;.354] | .653 [.638;.668] | .887 [.878;.897] | .982 [.978;.986] |
| | ZCP-sum | .049 [.043;.056] | .110 [.101;.121] | .302 [.288;.317] | .604 [.590;.620] | .866 [.855;.876] | .974 [.969;.979] |
| | ZCP-poly | .052 [.046;.060] | .128 [.119;.139] | .338 [.324;.353] | .651 [.637;.666] | .886 [.876;.896] | .983 [.979;.987] |
| | gANOVA | .051 [.045;.059] | .130 [.120;.141] | .340 [.325;.355] | .653 [.638;.668] | .888 [.878;.897] | .982 [.978;.986] |
| As | RI | .085 [.077;.094] | .174 [.163;.187] | .472 [.457;.488] | .797 [.784;.809] | .955 [.949;.961] | .996 [.993;.998] |
| | RI-L | .049 [.043;.056] | .116 [.106;.126] | .379 [.364;.394] | .724 [.711;.738] | .938 [.931;.945] | .992 [.990;.995] |
| | ZCP-sum | .048 [.042;.055] | .098 [.089;.107] | .317 [.303;.332] | .654 [.640;.669] | .907 [.898;.916] | .986 [.983;.990] |
| | ZCP-poly | .051 [.045;.058] | .116 [.106;.126] | .378 [.364;.394] | .723 [.709;.737] | .938 [.930;.945] | .993 [.990;.995] |
| | gANOVA | .050 [.043;.057] | .116 [.107;.127] | .379 [.364;.394] | .724 [.711;.738] | .938 [.930;.945] | .992 [.990;.995] |
| Am | RI | .443 [.428;.459] | .611 [.596;.626] | .878 [.868;.889] | .983 [.979;.987] | .999 [.998;1] | 1 [1;1] |
| | RI-L | .056 [.049;.064] | .140 [.130;.151] | .444 [.429;.459] | .794 [.782;.807] | .962 [.957;.968] | .997 [.996;.999] |
| | ZCP-sum | .072 [.065;.081] | .122 [.113;.133] | .315 [.301;.329] | .649 [.634;.664] | .896 [.886;.905] | .988 [.984;.991] |
| | ZCP-poly | .061 [.054;.069] | .147 [.136;.158] | .443 [.428;.458] | .794 [.782;.807] | .960 [.954;.966] | .997 [.996;.999] |
| | gANOVA | .056 [.049;.064] | .140 [.130;.151] | .443 [.428;.459] | .794 [.782;.807] | .962 [.957;.968] | .997 [.996;.999] |
| Ap:As | RI | .815 [.803;.827] | .856 [.845;.867] | .936 [.928;.944] | .986 [.983;.990] | .999 [.998;1] | 1 [1;1] |
| | RI-L | .040 [.034;.046] | .074 [.067;.083] | .190 [.178;.203] | .432 [.416;.447] | .701 [.687;.715] | .906 [.897;.915] |
| | ZCP-sum | .040 [.034;.046] | .053 [.046;.060] | .100 [.092;.110] | .217 [.204;.230] | .410 [.395;.425] | .651 [.637;.666] |
| | ZCP-poly | .047 [.041;.054] | .079 [.071;.088] | .200 [.188;.213] | .431 [.416;.446] | .702 [.687;.716] | .900 [.891;.910] |
| | gANOVA | .040 [.034;.046] | .074 [.066;.083] | .190 [.178;.202] | .430 [.415;.446] | .701 [.687;.715] | .906 [.897;.915] |
| Ap:Am | RI | .471 [.456;.487] | .564 [.549;.579] | .766 [.753;.779] | .931 [.923;.939] | .987 [.983;.990] | 1 [.999;1] |
| | RI-L | .056 [.049;.064] | .101 [.092;.111] | .261 [.247;.275] | .526 [.510;.541] | .798 [.786;.811] | .946 [.940;.953] |
| | ZCP-sum | .070 [.062;.078] | .092 [.084;.102] | .186 [.174;.198] | .363 [.348;.378] | .614 [.599;.630] | .831 [.819;.842] |
| | ZCP-poly | .058 [.051;.066] | .105 [.096;.115] | .272 [.259;.286] | .525 [.510;.540] | .788 [.775;.801] | .940 [.933;.947] |
| | gANOVA | .056 [.049;.064] | .101 [.092;.111] | .260 [.247;.274] | .525 [.510;.540] | .798 [.786;.811] | .946 [.940;.953] |
| As:Am | RI | .411 [.396;.427] | .573 [.558;.589] | .850 [.839;.861] | .980 [.976;.984] | .999 [.998;1] | 1 [1;1] |
| | RI-L | .061 [.054;.069] | .139 [.129;.150] | .403 [.388;.418] | .755 [.742;.769] | .957 [.951;.963] | .996 [.994;.998] |
| | ZCP-sum | .084 [.076;.093] | .128 [.119;.139] | .295 [.281;.309] | .591 [.576;.606] | .860 [.849;.871] | .976 [.972;.981] |
| | ZCP-poly | .068 [.061;.076] | .144 [.133;.155] | .405 [.390;.420] | .755 [.742;.769] | .955 [.949;.961] | .996 [.994;.998] |
| | gANOVA | .061 [.054;.069] | .139 [.129;.150] | .402 [.388;.418] | .754 [.741;.768] | .957 [.950;.963] | .996 [.994;.998] |
| Ap:As:Am | RI | .114 [.104;.124] | .150 [.140;.162] | .261 [.247;.275] | .466 [.451;.482] | .696 [.681;.710] | .888 [.878;.898] |
| | RI-L | .082 [.073;.090] | .105 [.096;.115] | .193 [.181;.206] | .360 [.345;.375] | .582 [.567;.598] | .791 [.778;.803] |
| | ZCP-sum | .082 [.074;.091] | .100 [.091;.110] | .159 [.148;.170] | .263 [.250;.277] | .443 [.428;.458] | .634 [.620;.650] |
| | ZCP-poly | .069 [.062;.077] | .089 [.081;.098] | .172 [.161;.184] | .328 [.313;.342] | .551 [.536;.566] | .768 [.755;.781] |
| | gANOVA | .082 [.073;.090] | .105 [.096;.115] | .193 [.181;.206] | .360 [.345;.375] | .582 [.567;.597] | .791 [.778;.803] |

Table S28: Power analysis of model M2 (see Table 2): The data are simulated using correlated random effects, without the interaction participants:stimuli. The estimated models include the random effects associated to the interaction participants:stimuli.

| variable | model | H0 | 0.2 | 0.4 | 0.6 | 0.8 | 1.0 |
|---|---|---|---|---|---|---|---|
| Ap | RI | .076 [.069;.085] | .169 [.158;.181] | .390 [.375;.405] | .706 [.692;.720] | .910 [.901;.919] | .990 [.987;.993] |
| | RI-L | .054 [.047;.061] | .134 [.123;.144] | .346 [.331;.361] | .658 [.644;.673] | .890 [.881;.900] | .984 [.980;.988] |
| | ZCP-sum | .052 [.045;.059] | .121 [.111;.131] | .315 [.301;.329] | .620 [.605;.635] | .871 [.860;.881] | .978 [.973;.983] |
| | ZCP-poly | .054 [.048;.062] | .134 [.123;.144] | .344 [.330;.359] | .656 [.641;.670] | .890 [.881;.900] | .984 [.980;.988] |
| | gANOVA | .054 [.047;.061] | .133 [.122;.143] | .346 [.331;.361] | .658 [.643;.673] | .890 [.881;.900] | .984 [.980;.988] |
| As | RI | .085 [.077;.094] | .174 [.163;.187] | .472 [.457;.488] | .797 [.784;.809] | .955 [.949;.961] | .996 [.993;.998] |
| | RI-L | .052 [.046;.060] | .121 [.112;.132] | .386 [.371;.401] | .730 [.717;.744] | .939 [.932;.947] | .993 [.990;.995] |
| | ZCP-sum | .051 [.045;.058] | .104 [.095;.114] | .334 [.319;.349] | .672 [.658;.687] | .914 [.905;.923] | .988 [.984;.991] |
| | ZCP-poly | .054 [.047;.061] | .121 [.111;.131] | .385 [.370;.401] | .730 [.717;.744] | .940 [.932;.947] | .993 [.990;.996] |
| | gANOVA | .053 [.046;.060] | .122 [.112;.132] | .387 [.372;.402] | .730 [.717;.744] | .939 [.932;.947] | .993 [.990;.995] |
| Am | RI | .536 [.520;.551] | .691 [.677;.705] | .909 [.900;.918] | .989 [.986;.992] | 1 [.999;1] | 1 [1;1] |
| | RI-L | .052 [.045;.059] | .132 [.122;.143] | .428 [.413;.444] | .784 [.772;.797] | .962 [.956;.968] | .997 [.995;.999] |
| | ZCP-sum | .067 [.060;.075] | .108 [.099;.118] | .285 [.272;.300] | .621 [.606;.636] | .880 [.871;.891] | .983 [.979;.987] |
| | ZCP-poly | .056 [.049;.063] | .139 [.128;.150] | .430 [.415;.445] | .784 [.771;.797] | .958 [.951;.964] | .997 [.995;.999] |
| | gANOVA | .052 [.045;.059] | .133 [.122;.143] | .428 [.413;.444] | .784 [.772;.797] | .962 [.956;.968] | .997 [.995;.999] |
| Ap:As | RI | .670 [.656;.685] | .736 [.722;.749] | .866 [.856;.877] | .966 [.960;.971] | .995 [.993;.997] | 1 [.999;1] |
| | RI-L | .046 [.040;.053] | .085 [.077;.094] | .205 [.193;.218] | .452 [.437;.467] | .718 [.704;.732] | .916 [.907;.924] |
| | ZCP-sum | .052 [.045;.059] | .068 [.061;.076] | .128 [.118;.138] | .260 [.247;.274] | .476 [.460;.491] | .714 [.700;.728] |
| | ZCP-poly | .055 [.048;.063] | .090 [.082;.100] | .216 [.204;.229] | .456 [.441;.472] | .724 [.710;.738] | .911 [.902;.920] |
| | gANOVA | .046 [.040;.053] | .084 [.076;.093] | .205 [.193;.218] | .451 [.435;.466] | .718 [.704;.732] | .915 [.906;.924] |
| Ap:Am | RI | .597 [.582;.613] | .678 [.664;.693] | .840 [.829;.851] | .959 [.953;.965] | .993 [.990;.996] | 1 [.999;1] |
| | RI-L | .046 [.040;.053] | .088 [.079;.097] | .238 [.226;.252] | .498 [.483;.514] | .783 [.770;.796] | .940 [.933;.948] |
| | ZCP-sum | .067 [.060;.075] | .088 [.079;.097] | .169 [.158;.181] | .333 [.319;.348] | .568 [.553;.584] | .799 [.787;.811] |
| | ZCP-poly | .054 [.047;.061] | .098 [.089;.107] | .254 [.240;.267] | .505 [.490;.521] | .776 [.763;.789] | .935 [.927;.943] |
| | gANOVA | .046 [.040;.053] | .088 [.079;.097] | .238 [.226;.252] | .497 [.482;.513] | .782 [.770;.795] | .939 [.932;.947] |
| As:Am | RI | .543 [.528;.559] | .699 [.685;.713] | .908 [.899;.917] | .989 [.985;.992] | 1 [.999;1] | 1 [1;1] |
| | RI-L | .052 [.045;.059] | .121 [.111;.131] | .380 [.365;.395] | .736 [.722;.750] | .950 [.943;.957] | .996 [.994;.998] |
| | ZCP-sum | .078 [.070;.087] | .116 [.106;.126] | .258 [.245;.272] | .537 [.522;.553] | .822 [.810;.834] | .968 [.963;.974] |
| | ZCP-poly | .061 [.054;.069] | .130 [.120;.141] | .384 [.369;.399] | .741 [.728;.755] | .950 [.943;.957] | .995 [.993;.997] |
| | gANOVA | .052 [.045;.059] | .121 [.111;.131] | .380 [.365;.395] | .735 [.722;.749] | .949 [.943;.956] | .996 [.994;.998] |
| Ap:As:Am | RI | .256 [.243;.270] | .298 [.284;.312] | .448 [.433;.464] | .664 [.650;.679] | .845 [.834;.856] | .959 [.953;.965] |
| | RI-L | .055 [.049;.063] | .074 [.066;.082] | .138 [.128;.149] | .288 [.274;.302] | .506 [.490;.521] | .740 [.727;.754] |
| | ZCP-sum | .080 [.072;.089] | .092 [.083;.101] | .132 [.122;.143] | .212 [.199;.225] | .352 [.338;.367] | .531 [.515;.546] |
| | ZCP-poly | .058 [.052;.066] | .080 [.072;.089] | .144 [.134;.156] | .289 [.276;.304] | .513 [.498;.529] | .730 [.716;.744] |
| | gANOVA | .055 [.049;.063] | .074 [.066;.082] | .138 [.128;.149] | .288 [.274;.302] | .506 [.491;.522] | .739 [.726;.753] |

Table S29: Power analysis of model M2 (see Table 2): The data are simulated using correlated random effects, with the interaction participants:stimuli. The estimated models do not include the random effects associated to the interaction participants:stimuli.

| variable | model | H0 | 0.2 | 0.4 | 0.6 | 0.8 | 1.0 |
|---|---|---|---|---|---|---|---|
| Ap | RI | .080 [.072;.089] | .164 [.152;.175] | .408 [.393;.423] | .723 [.709;.737] | .918 [.909;.926] | .989 [.985;.992] |
| | RI-L | .058 [.051;.066] | .128 [.118;.139] | .352 [.338;.367] | .674 [.660;.689] | .900 [.890;.909] | .983 [.979;.987] |
| | ZCP-sum | .053 [.046;.060] | .114 [.105;.124] | .313 [.299;.328] | .634 [.619;.649] | .883 [.873;.893] | .976 [.972;.981] |
| | ZCP-poly | .059 [.052;.066] | .128 [.118;.139] | .353 [.338;.368] | .673 [.659;.688] | .900 [.890;.909] | .984 [.980;.988] |
| | gANOVA | .058 [.051;.066] | .128 [.118;.139] | .352 [.338;.367] | .675 [.660;.689] | .900 [.890;.909] | .983 [.979;.987] |
| As | RI | .086 [.077;.095] | .183 [.171;.195] | .476 [.461;.492] | .802 [.789;.814] | .961 [.955;.967] | .996 [.993;.998] |
| | RI-L | .048 [.042;.055] | .127 [.117;.137] | .386 [.371;.401] | .739 [.726;.753] | .943 [.936;.950] | .993 [.991;.996] |
| | ZCP-sum | .047 [.041;.054] | .104 [.095;.114] | .326 [.312;.341] | .677 [.663;.692] | .921 [.913;.929] | .989 [.986;.992] |
| | ZCP-poly | .049 [.042;.056] | .126 [.116;.137] | .389 [.374;.404] | .737 [.723;.750] | .941 [.933;.948] | .993 [.991;.996] |
| | gANOVA | .048 [.042;.055] | .127 [.117;.137] | .386 [.371;.402] | .740 [.726;.753] | .943 [.936;.950] | .993 [.991;.996] |
| Am | RI | .528 [.513;.544] | .679 [.664;.693] | .899 [.890;.908] | .987 [.983;.991] | .998 [.997;1] | 1 [1;1] |
| | RI-L | .049 [.043;.056] | .147 [.137;.159] | .446 [.431;.462] | .794 [.782;.807] | .963 [.957;.969] | .996 [.995;.998] |
| | ZCP-sum | .068 [.060;.076] | .119 [.109;.129] | .315 [.301;.329] | .629 [.614;.644] | .890 [.880;.899] | .982 [.978;.986] |
| | ZCP-poly | .054 [.047;.061] | .151 [.140;.162] | .447 [.432;.463] | .796 [.784;.809] | .964 [.959;.970] | .996 [.995;.998] |
| | gANOVA | .048 [.042;.056] | .147 [.136;.158] | .446 [.430;.461] | .794 [.782;.807] | .963 [.957;.969] | .996 [.995;.998] |
| Ap:As | RI | .834 [.823;.846] | .877 [.867;.887] | .957 [.950;.963] | .990 [.987;.993] | 1 [1;1] | 1 [1;1] |
| | RI-L | .050 [.044;.058] | .092 [.084;.102] | .234 [.221;.248] | .490 [.475;.505] | .774 [.761;.787] | .936 [.928;.943] |
| | ZCP-sum | .049 [.043;.056] | .064 [.057;.072] | .123 [.113;.134] | .253 [.240;.267] | .472 [.457;.487] | .719 [.705;.733] |
| | ZCP-poly | .059 [.052;.067] | .096 [.087;.106] | .245 [.232;.259] | .492 [.477;.508] | .768 [.755;.781] | .934 [.927;.942] |
| | gANOVA | .050 [.044;.058] | .092 [.084;.102] | .234 [.221;.247] | .489 [.474;.505] | .774 [.761;.787] | .935 [.928;.943] |
| Ap:Am | RI | .555 [.540;.571] | .647 [.633;.662] | .833 [.822;.845] | .958 [.952;.964] | .996 [.994;.998] | 1 [1;1] |
| | RI-L | .053 [.046;.060] | .092 [.084;.102] | .248 [.235;.262] | .519 [.504;.535] | .787 [.775;.800] | .948 [.941;.955] |
| | ZCP-sum | .069 [.061;.077] | .087 [.078;.096] | .166 [.155;.178] | .346 [.331;.361] | .573 [.558;.589] | .809 [.797;.821] |
| | ZCP-poly | .058 [.051;.066] | .102 [.093;.112] | .254 [.241;.268] | .519 [.503;.534] | .782 [.770;.795] | .945 [.938;.952] |
| | gANOVA | .052 [.046;.060] | .093 [.084;.102] | .248 [.235;.262] | .519 [.503;.534] | .786 [.774;.799] | .946 [.940;.953] |
| As:Am | RI | .500 [.485;.516] | .655 [.640;.670] | .882 [.872;.892] | .985 [.982;.989] | 1 [.999;1] | 1 [1;1] |
| | RI-L | .048 [.042;.055] | .122 [.112;.133] | .395 [.380;.410] | .745 [.731;.758] | .948 [.941;.954] | .996 [.994;.998] |
| | ZCP-sum | .066 [.059;.074] | .107 [.098;.117] | .251 [.238;.265] | .543 [.528;.559] | .820 [.808;.832] | .960 [.954;.966] |
| | ZCP-poly | .057 [.050;.064] | .130 [.120;.141] | .401 [.386;.417] | .740 [.726;.754] | .943 [.936;.950] | .995 [.993;.997] |
| | gANOVA | .048 [.042;.055] | .122 [.112;.133] | .395 [.380;.410] | .744 [.731;.758] | .947 [.940;.954] | .996 [.994;.998] |
| Ap:As:Am | RI | .192 [.181;.205] | .240 [.227;.253] | .371 [.356;.386] | .583 [.568;.599] | .804 [.792;.816] | .939 [.932;.946] |
| | RI-L | .058 [.051;.066] | .076 [.068;.085] | .150 [.140;.162] | .296 [.283;.311] | .516 [.501;.532] | .749 [.735;.762] |
| | ZCP-sum | .087 [.078;.096] | .099 [.090;.109] | .141 [.131;.152] | .229 [.216;.242] | .353 [.338;.368] | .528 [.513;.543] |
| | ZCP-poly | .063 [.056;.071] | .083 [.075;.092] | .159 [.148;.171] | .306 [.292;.321] | .525 [.510;.541] | .752 [.739;.766] |
| | gANOVA | .058 [.052;.066] | .076 [.068;.085] | .150 [.140;.162] | .296 [.283;.311] | .516 [.501;.532] | .748 [.735;.762] |

Table S30: Power analysis of model M2 (see Table 2): The data are simulated using correlated random effects, with the interaction participants:stimuli. The estimated models include the random effects associated to the interaction participants:stimuli.

| variable | model | H0 | 0.2 | 0.4 | 0.6 | 0.8 | 1.0 |
|---|---|---|---|---|---|---|---|
| Ap | RI | .080 [.072;.089] | .164 [.152;.175] | .408 [.393;.423] | .723 [.709;.737] | .918 [.909;.926] | .989 [.985;.992] |
| | RI-L | .059 [.052;.066] | .128 [.118;.139] | .353 [.338;.368] | .675 [.660;.689] | .900 [.890;.909] | .983 [.979;.987] |
| | ZCP-sum | .053 [.047;.061] | .114 [.105;.125] | .314 [.300;.328] | .635 [.620;.650] | .883 [.873;.893] | .976 [.972;.981] |
| | ZCP-poly | .058 [.052;.066] | .129 [.119;.139] | .353 [.339;.368] | .673 [.659;.688] | .900 [.890;.909] | .984 [.980;.988] |
| | gANOVA | .058 [.051;.066] | .128 [.118;.139] | .353 [.338;.368] | .675 [.661;.690] | .900 [.890;.909] | .983 [.979;.987] |
| As | RI | .086 [.077;.095] | .183 [.171;.195] | .476 [.461;.492] | .802 [.789;.814] | .961 [.955;.967] | .996 [.993;.998] |
| | RI-L | .048 [.042;.055] | .127 [.117;.138] | .386 [.372;.402] | .740 [.727;.754] | .943 [.936;.950] | .993 [.991;.996] |
| | ZCP-sum | .047 [.041;.054] | .104 [.095;.114] | .326 [.312;.341] | .679 [.664;.693] | .922 [.914;.930] | .989 [.986;.992] |
| | ZCP-poly | .049 [.043;.056] | .126 [.116;.137] | .390 [.375;.405] | .737 [.724;.751] | .941 [.934;.948] | .994 [.991;.996] |
| | gANOVA | .048 [.042;.055] | .127 [.117;.138] | .387 [.372;.402] | .740 [.727;.754] | .943 [.936;.950] | .993 [.991;.996] |
| Am | RI | .575 [.560;.591] | .710 [.696;.724] | .914 [.906;.923] | .989 [.986;.992] | .999 [.998;1] | 1 [1;1] |
| | RI-L | .048 [.042;.055] | .147 [.137;.159] | .445 [.430;.461] | .794 [.781;.806] | .963 [.957;.969] | .996 [.995;.998] |
| | ZCP-sum | .068 [.060;.076] | .118 [.108;.128] | .314 [.300;.328] | .628 [.613;.643] | .888 [.879;.898] | .982 [.978;.986] |
| | ZCP-poly | .053 [.047;.061] | .150 [.140;.162] | .446 [.431;.462] | .796 [.784;.809] | .964 [.959;.970] | .996 [.995;.998] |
| | gANOVA | .048 [.042;.055] | .147 [.136;.158] | .444 [.429;.460] | .794 [.781;.806] | .963 [.957;.969] | .996 [.995;.998] |
| Ap:As | RI | .762 [.749;.775] | .826 [.814;.837] | .932 [.924;.940] | .982 [.978;.986] | .999 [.998;1] | 1 [1;1] |
| | RI-L | .051 [.044;.058] | .093 [.084;.102] | .235 [.223;.249] | .492 [.477;.508] | .775 [.762;.788] | .935 [.928;.943] |
| | ZCP-sum | .050 [.043;.057] | .065 [.058;.073] | .124 [.114;.135] | .255 [.241;.268] | .474 [.459;.490] | .721 [.707;.735] |
| | ZCP-poly | .059 [.052;.067] | .097 [.088;.106] | .247 [.234;.261] | .494 [.478;.509] | .770 [.757;.783] | .935 [.928;.943] |
| | gANOVA | .051 [.044;.058] | .093 [.084;.102] | .235 [.222;.249] | .492 [.477;.507] | .775 [.762;.788] | .935 [.928;.943] |
| Ap:Am | RI | .609 [.594;.625] | .696 [.682;.711] | .866 [.856;.877] | .968 [.963;.974] | .996 [.995;.998] | 1 [1;1] |
| | RI-L | .052 [.046;.059] | .093 [.084;.102] | .247 [.234;.260] | .517 [.502;.533] | .786 [.773;.798] | .948 [.941;.955] |
| | ZCP-sum | .068 [.060;.076] | .087 [.078;.096] | .165 [.154;.177] | .343 [.329;.358] | .570 [.555;.586] | .807 [.795;.819] |
| | ZCP-poly | .057 [.050;.065] | .101 [.092;.111] | .253 [.240;.267] | .517 [.502;.533] | .780 [.768;.793] | .944 [.937;.951] |
| | gANOVA | .051 [.045;.059] | .092 [.084;.102] | .246 [.234;.260] | .517 [.501;.532] | .785 [.772;.798] | .946 [.940;.953] |
| As:Am | RI | .574 [.558;.589] | .703 [.689;.717] | .905 [.896;.914] | .988 [.985;.991] | 1 [.999;1] | 1 [1;1] |
| | RI-L | .048 [.041;.055] | .121 [.111;.131] | .394 [.379;.409] | .744 [.731;.758] | .947 [.940;.954] | .996 [.994;.998] |
| | ZCP-sum | .065 [.058;.073] | .106 [.097;.116] | .249 [.236;.263] | .541 [.526;.557] | .817 [.805;.829] | .958 [.952;.964] |
| | ZCP-poly | .056 [.050;.064] | .129 [.119;.140] | .400 [.385;.415] | .739 [.725;.752] | .942 [.935;.949] | .995 [.993;.997] |
| | gANOVA | .048 [.042;.055] | .120 [.111;.131] | .393 [.378;.409] | .744 [.731;.758] | .946 [.940;.953] | .996 [.994;.998] |
| Ap:As:Am | RI | .270 [.257;.285] | .323 [.309;.338] | .462 [.447;.477] | .679 [.664;.693] | .863 [.853;.874] | .962 [.956;.968] |
| | RI-L | .057 [.050;.065] | .075 [.067;.083] | .148 [.138;.160] | .293 [.280;.308] | .512 [.497;.528] | .746 [.733;.760] |
| | ZCP-sum | .084 [.076;.093] | .098 [.089;.108] | .139 [.129;.150] | .225 [.213;.239] | .350 [.335;.365] | .520 [.505;.536] |
| | ZCP-poly | .062 [.055;.070] | .082 [.074;.091] | .156 [.146;.168] | .302 [.288;.317] | .520 [.505;.536] | .749 [.735;.762] |
| | gANOVA | .057 [.050;.065] | .075 [.067;.084] | .148 [.138;.160] | .293 [.279;.307] | .512 [.497;.528] | .746 [.733;.760] |

# 3 Results of simulation: gANOVA vs RI-L

Table S31: Type I error rate of design M1 where the data are generated without random intercepts. Subset of data simulated using 18 participants and 18 stimuli.

| | | | RI-L | RI-L+ | gANOVA | gANOVA+ |
|---|---|---|---|---|---|---|
| Ap | corr. | no PT:SM | *.023 [.019;.028]* | *.023 [.019;.028]* | **.045 [.039;.052]** | **.045 [.039;.052]** |
| | | PT:SM | *.026 [.021;.031]* | *.026 [.021;.031]* | **.051 [.045;.058]** | **.051 [.045;.059]** |
| | spheric. | no PT:SM | *.018 [.015;.023]* | *.018 [.015;.023]* | **.048 [.042;.055]** | **.048 [.042;.055]** |
| | | PT:SM | *.021 [.017;.026]* | *.021 [.017;.026]* | **.044 [.038;.051]** | **.044 [.038;.051]** |
| As | corr. | no PT:SM | *.034 [.029;.040]* | *.034 [.029;.040]* | **.051 [.045;.059]** | **.051 [.045;.059]** |
| | | PT:SM | *.040 [.035;.047]* | *.040 [.034;.047]* | **.051 [.045;.059]** | **.051 [.045;.059]** |
| | spheric. | no PT:SM | *.036 [.030;.042]* | *.036 [.030;.042]* | **.052 [.045;.059]** | **.052 [.045;.059]** |
| | | PT:SM | *.042 [.036;.048]* | *.041 [.036;.048]* | **.050 [.043;.057]** | **.050 [.043;.057]** |
| Am | corr. | no PT:SM | .120 [.110;.131] | .120 [.110;.131] | **.050 [.044;.058]** | **.050 [.044;.058]** |
| | | PT:SM | .115 [.106;.126] | .115 [.106;.125] | **.051 [.044;.058]** | **.050 [.044;.058]** |
| | spheric. | no PT:SM | .113 [.104;.124] | .113 [.104;.124] | **.050 [.044;.058]** | **.050 [.044;.058]** |
| | | PT:SM | .105 [.096;.115] | .105 [.096;.115] | **.051 [.045;.059]** | **.051 [.045;.058]** |
| Ap:As | corr. | no PT:SM | .112 [.102;.122] | .112 [.102;.122] | **.048 [.042;.055]** | **.048 [.042;.055]** |
| | | PT:SM | .106 [.097;.116] | .106 [.097;.116] | **.044 [.039;.051]** | **.044 [.039;.051]** |
| | spheric. | no PT:SM | .109 [.100;.119] | .109 [.100;.119] | **.049 [.043;.056]** | **.049 [.043;.056]** |
| | | PT:SM | .110 [.100;.120] | .109 [.100;.119] | **.050 [.043;.057]** | **.050 [.043;.057]** |
| Ap:Am | corr. | no PT:SM | .082 [.074;.091] | .082 [.074;.091] | **.051 [.045;.058]** | **.051 [.045;.058]** |
| | | PT:SM | .079 [.071;.088] | .079 [.071;.088] | **.050 [.044;.058]** | **.050 [.044;.057]** |
| | spheric. | no PT:SM | .079 [.071;.088] | .079 [.071;.088] | **.052 [.046;.059]** | **.052 [.046;.059]** |
| | | PT:SM | .080 [.072;.088] | .079 [.071;.088] | **.050 [.044;.058]** | **.050 [.044;.057]** |
| As:Am | corr. | no PT:SM | .066 [.059;.074] | .066 [.059;.074] | **.044 [.038;.051]** | **.044 [.038;.051]** |
| | | PT:SM | .068 [.061;.076] | .068 [.061;.076] | **.047 [.041;.054]** | **.047 [.041;.054]** |
| | spheric. | no PT:SM | .083 [.075;.092] | .083 [.075;.092] | .060 [.053;.068] | .060 [.053;.068] |
| | | PT:SM | .083 [.075;.092] | .083 [.075;.092] | .060 [.053;.067] | .060 [.053;.067] |
| Ap:As:Am | corr. | no PT:SM | *.036 [.031;.043]* | *.036 [.031;.043]* | *.042 [.037;.049]* | *.042 [.037;.049]* |
| | | PT:SM | *.038 [.033;.045]* | *.038 [.033;.045]* | **.051 [.045;.059]** | **.051 [.045;.058]** |
| | spheric. | no PT:SM | *.035 [.030;.041]* | *.035 [.030;.041]* | *.044 [.038;.050]* | *.044 [.038;.050]* |
| | | PT:SM | *.035 [.030;.041]* | *.035 [.030;.041]* | **.045 [.039;.052]** | **.045 [.039;.052]** |

Table S32: Type I error rate of design M1 where the data are generated without random intercepts. Subset of data simulated using 18 participants and 36 stimuli.

| | | | RI-L | RI-L+ | gANOVA | gANOVA+ |
|---|---|---|---|---|---|---|
| Ap | corr. | no PT:SM | *.005 [.003;.008]* | *.005 [.003;.008]* | **.046 [.040;.054]** | **.046 [.040;.054]** |
| | | PT:SM | *.006 [.004;.008]* | *.006 [.004;.008]* | **.049 [.043;.056]** | **.049 [.043;.056]** |
| | spheric. | no PT:SM | *.006 [.004;.008]* | *.006 [.004;.008]* | **.051 [.045;.058]** | **.051 [.045;.058]** |
| | | PT:SM | *.005 [.003;.008]* | *.005 [.003;.008]* | *.039 [.033;.045]* | *.039 [.033;.045]* |
| As | corr. | no PT:SM | .064 [.057;.072] | .064 [.057;.072] | **.048 [.042;.056]** | **.048 [.042;.056]** |
| | | PT:SM | .066 [.059;.074] | .066 [.058;.074] | **.050 [.044;.057]** | **.050 [.044;.058]** |
| | spheric. | no PT:SM | .061 [.054;.069] | .062 [.054;.069] | **.048 [.041;.055]** | **.048 [.041;.055]** |
| | | PT:SM | .063 [.056;.071] | .062 [.055;.070] | **.047 [.041;.054]** | **.047 [.041;.054]** |
| Am | corr. | no PT:SM | .119 [.109;.129] | .119 [.109;.129] | **.047 [.041;.054]** | **.047 [.041;.054]** |
| | | PT:SM | .118 [.108;.128] | .118 [.108;.128] | **.050 [.043;.057]** | **.050 [.043;.057]** |
| | spheric. | no PT:SM | .117 [.107;.127] | .117 [.107;.127] | **.046 [.040;.054]** | **.046 [.040;.054]** |
| | | PT:SM | .107 [.098;.117] | .107 [.098;.117] | **.051 [.044;.058]** | **.051 [.044;.058]** |
| Ap:As | corr. | no PT:SM | .114 [.105;.125] | .114 [.105;.125] | **.052 [.045;.059]** | **.052 [.045;.059]** |
| | | PT:SM | .114 [.104;.124] | .113 [.104;.123] | **.050 [.044;.058]** | **.050 [.044;.058]** |
| | spheric. | no PT:SM | .113 [.103;.123] | .113 [.103;.123] | **.047 [.041;.054]** | **.047 [.041;.054]** |
| | | PT:SM | .111 [.101;.121] | .110 [.101;.121] | **.050 [.044;.058]** | **.050 [.044;.058]** |
| Ap:Am | corr. | no PT:SM | .095 [.086;.104] | .095 [.086;.104] | **.051 [.045;.058]** | **.051 [.045;.058]** |
| | | PT:SM | .099 [.090;.109] | .099 [.090;.108] | **.051 [.045;.059]** | **.051 [.045;.059]** |
| | spheric. | no PT:SM | .092 [.083;.101] | .092 [.083;.101] | **.052 [.045;.059]** | **.052 [.045;.059]** |
| | | PT:SM | .089 [.081;.099] | .089 [.081;.099] | **.052 [.046;.060]** | **.052 [.046;.060]** |
| As:Am | corr. | no PT:SM | .056 [.050;.064] | .056 [.050;.064] | **.048 [.042;.055]** | **.048 [.042;.055]** |
| | | PT:SM | **.055 [.049;.063]** | **.055 [.049;.063]** | **.048 [.041;.055]** | **.048 [.041;.055]** |
| | spheric. | no PT:SM | .059 [.052;.067] | .059 [.052;.067] | **.048 [.042;.055]** | **.048 [.042;.055]** |
| | | PT:SM | .058 [.052;.066] | .058 [.051;.066] | **.051 [.045;.058]** | **.051 [.045;.058]** |
| Ap:As:Am | corr. | no PT:SM | *.040 [.035;.047]* | *.040 [.034;.047]* | **.052 [.045;.059]** | **.052 [.045;.059]** |
| | | PT:SM | *.037 [.032;.043]* | *.037 [.032;.043]* | **.051 [.045;.059]** | **.051 [.045;.059]** |
| | spheric. | no PT:SM | *.033 [.028;.039]* | *.033 [.028;.039]* | **.047 [.041;.054]** | **.047 [.041;.054]** |
| | | PT:SM | *.032 [.027;.038]* | *.032 [.027;.038]* | **.048 [.042;.056]** | **.048 [.042;.055]** |
